# Supplementary material for: Robust improper maximum likelihood: tuning, computation, and a comparison with other methods for robust Gaussian clustering
Source: arXiv:1406.0808 ancillary file (2017-01-28)
Supplement: Supplementary file 1 [file supplement.pdf]

SUPPLEMENT TO

# Robust Improper Maximum Likelihood: Tuning, Computation, and a Comparison With Other Methods for Robust Gaussian Clustering


Pietro Coretto*
University of Salerno, Italy
e-mail: pcoretto@unisa.it

Christian Hennig†
University College London, UK
e-mail: c.hennig@ucl.ac.uk


The present manuscript contains material that is supplementary to Coretto and Hennig (2015). Unless otherwise stated, notation refers to the main paper.

## Contents


1 Methods from the literature 2

2 RIMLE/OTRILME computing 4

2.1 RIMLE numerical approximation . . . . . . . . . . . . . . . . . . . . . . . . . . . 4

2.2 OTRIMLE numerical approximation . . . . . . . . . . . . . . . . . . . . . . . . . 5

2.3 Choice of initial values . . . . . . . . . . . . . . . . . . . . . . . . . . . . . . . . . 6

2.4 Computation of the MCD functional . . . . . . . . . . . . . . . . . . . . . . . . . 8

2.5 Additional remarks for the computation of misclassification rates . . . . . . . . . 8

3 Definition of DGPs 8

4 Plots for the DGPs and misclassification rates from the simulation study 12

5 Detailed summary tables for the simulation study 24

6 Plots for the analysis of Dortmund data 28



*The author gratefully acknowledges support from the Univeristy of Salerno grant program "Sistema di calcolo ad alte prestazioni per l'analisi economica, finanziaria e statistica (HPC - High Performance Computing) - prot. ASSA098434, 2009"

†The author gratefully acknowledges support from the EPSRC grant EP/K033972/1.

**7 Information on folk song data** **33**

7.1 Features . . . . . . . . . . . . . . . . . . . . . . . . . . . . . . . . . . . . . . 33

7.2 Plot . . . . . . . . . . . . . . . . . . . . . . . . . . . . . . . . . . . . . . . . 33

**References** **33**

# 1 Methods from the literature

Here is a more detailed description of some robust clustering methods from the literature that were presented in Section 2 of Coretto and Hennig (2015) that are used in the simulation study.

In order to settle the notation, we repeat some bits of Section 2 of Coretto and Hennig (2015). In the following, assume an observed sample $\underline{x_n} = \{x_1, x_2, \ldots, x_n\}$, where $x_i$ is the realization of a random variable $X_i \in \mathbb{R}^p$ with $p \geq 1$; $X_1, \ldots, X_n$ i.i.d. The goal is to cluster the sample points into $G$ distinct groups.

**Maximum Likelihood (ML) for Gaussian mixtures (gmix).** Let $\phi(x; \mu, \Sigma)$ be the density of a multivariate Gaussian distribution with mean vector $\mu \in \mathbb{R}^p$ and $p \times p$ covariance matrix $\Sigma$. Assume that the observed sample is i.i.d. drawn from the finite Gaussian mixture distribution having density

$$m(x; \theta) = \sum_{j=1}^{G} \pi_j \phi(x; \mu_j, \Sigma_j), \tag{1.1}$$

where $\pi_j \in [0, 1]$ for all $j = 1, 2, \ldots, G$ and $\sum_{j=1}^{G} \pi_j = 1$, $\theta$ is the parameter vector containing the triplets $\pi_j, \mu_j, \Sigma_j$ for all $j = 1, 2, \ldots, G$. Clustering coincides with assigning points to the mixture components based on ML parameter estimates. $\pi_j$ can be interpreted as the expected proportion of points originated from the $j$th component. Let $\theta_n^{\text{ml}}$ be the ML estimator for $\theta$. Let $\tau_{ij}^{\text{ml}}$ be the estimated posterior probability that the observed point $x_i$ has been drawn from the $j$th mixture component, i.e.,

$$\tau_{ij}^{\text{ml}} = \frac{\pi_{j,n}^{\text{ml}} \phi(x_i; \mu_{j,n}^{\text{ml}}, \Sigma_{j,n}^{\text{ml}})}{m(x_i; \theta_n^{\text{ml}})} \qquad \text{for all} \qquad j = 1, 2, \ldots, G. \tag{1.2}$$

The point $x_i$ can then be assigned to the $k$th cluster if $k = \arg\max_{j=1,2,\ldots,G} \tau_{ij}^{\text{ml}}$. This assignment method is common to all model-based clustering methods.

**ML–type estimator for Gaussian mixtures with uniform noise (gmix.u).** Banfield and Raftery (1993) suggested to accommodate "noise" such as outliers by adding a uniform mixture component to (1.1), calling it "*noise component*", which is implemented in the `mclust` package mentioned above. The resulting density for the data is

$$m_u(x; \theta) := \pi_0 \mathbb{1}\{x \in S\} \frac{1}{V_n} + \sum_{j=1}^{G} \pi_j \phi(x; \mu_j, \Sigma_j), \tag{1.3}$$

where $S \subset \mathbb{R}^p$ with volume $V_n$, $\pi_0 \in [0, 1)$, $\pi_0 + \sum_{j=1}^{G} \pi_j = 1$, $\theta$ now also includes $\pi_0$. The parameter $\pi_0$ represents the proportion of the uniform noise component. Banfield and Raftery (1993) proposed to fix $S$ as the convex hull of the data, although the `mclust` package actually uses a hyper-rectangle that includes $S$ (Coretto and Hennig (2011) noted that this does not normally yield a proper ML-estimator). $\theta$ is estimated by maximizing the log-likelihood function

corresponding to (1.3). Denoting this estimator $\theta_n^{\mathrm{ml}}$, the estimated posterior probability that a point $x_i$ belongs to the noise component is given by $\tau_{i0}^{\mathrm{ml}} = (\pi_{0,n}^{\mathrm{ml}}/V_n)/m_u(x_i;\theta_n^{\mathrm{ml}})$. Points are then assigned to clusters or the noise component as above. A drawback is that $V_n$ may seriously be affected by outlying points, reducing the formal breakdown point of the method to zero (Hennig, 2004).

**ML for mixtures of Student–t distributions (tmix).** McLachlan and Peel (2000b) propose to replace the Gaussian densities in (1.1) with multivariate Student-t densities, because they have heavier tails and can therefore accommodate outliers in a better way. Observations can be declared "noise" if they lie so far away from their cluster center that they are in a low density area with a probability lower than some pre-specified small $\alpha$. Let $f(x;\mu,S,v)$ be the non-central Student-t density in $\mathbb{R}^p$ with expectation $\mu$, positive definite scale matrix $S$, and $v$ degrees of freedom. Consider the density

$$m_t(x;\theta) := \sum_{j=1}^{G} \pi_j f(x;\mu_j,S_j,v_j), \tag{1.4}$$

where $\theta$ contains all mixture component parameters to be fitted by ML. Degrees of freedom can be fixed a priori or can be estimated. The unknown parameter vector is estimated by ML. A point $x_i$ assigned to the $j$th mixture component can be defined as outlier if

$$(x_i - \mu_j^{\mathrm{ml}})'(S_j^{\mathrm{ml}})^{-1}(x_i - \mu_j^{\mathrm{ml}}) \geq q(\alpha), \tag{1.5}$$

where $\mu_j^{\mathrm{ml}}$ and $S_j^{\mathrm{ml}}$ are the resulting ML estimates for the model (1.4). McLachlan and Peel (2000a) suggest $q(\alpha) = \chi^2_{p,(1-\alpha)}$, the $(1-\alpha)$-quantile of the $\chi^2$ distribution with $p$ degrees of freedom. Hennig (2004) showed that this method is not breakdown-robust.

**TCLUST.** Gallegos (2002) and Gallegos and Ritter (2005) proposed the "spurious outliers model" as a probabilistic framework for robust crisp cluster analysis based on Gaussian distributions (more recent theoretical results are given in Gallegos and Ritter (2013)). García-Escudero et al. (2008) proposed a modification allowing different clusters to have different weights. This amounts to maximizing the weighted likelihood function

$$\left\{\prod_{j=1}^{G}\prod_{i\in R_j} \pi_j \phi(x_i;\mu_j,\Sigma_j)\right\}\left\{\prod_{i\notin R} g_i(x_i)\right\}, \tag{1.6}$$

where $R = \cup_{j=1}^{G} R_j$ is the set of indexes of clustered observations with $\#\{R\} = [n(1-\alpha)]$, and $g_i(\cdot)$ are the densities modeling outlying observations, $\pi_j$ is the $j$th cluster's weight with $\pi_j \in [0,1]$ and $\sum_{j=1}^{G}\pi_j = 1$. Let $\theta$ be the unknown parameter vector including all triplets $\pi_j, \mu_j, \Sigma_j$ for all $j = 1,2,\ldots,G$ (in the original spurious outlier model, $\pi_j = 1\ \forall j$, defining a "fixed partition model" with parameters for the cluster membership of every point). $\alpha > 0$ is the trimming rate, i.e., the proportion of points interpreted as outliers/noise. The authors show that for maximization of (1.6) it suffices to maximize of the left-hand side term of (1.6) and to "trim" the outliers, so that the problem boils down to

$$\theta^{\mathrm{tclust}} := \underset{\theta\in\Theta,\#\{R\}=[n(1-\alpha)]}{\arg\max} \sum_{j=1}^{G}\sum_{i\in R_j} \left(\log \pi_j + \log \phi(x;\mu_j,\Sigma_j)\right). \tag{1.7}$$

As for the previously introduced methods, constraints will be discussed in detail in Section 3.1 in Coretto and Hennig (2015). Under mild regularity conditions, García-Escudero et al. (2008) propose an algorithm for computing $\theta_n^{\mathrm{tclust}}$ and provide consistency theory. The TCLUST methodology is implemented in R's `tclust` package by Fritz et al. (2012). Partition methods

with trimming started with the trimmed $k$-means proposal of Cuesta-Albertos et al. (1997).

# 2 RIMLE/OTRILME computing

In this section we provide details about computation of the RIMLE/OTRIMLE. We also give a detailed description of the initialization strategy adopted in the comparative Monte Carlo experiment. References to equations in brackets in this section are to Coretto and Hennig (2015).

## 2.1 RIMLE numerical approximation

Fix three computing parameters `em.tol, min.det, min.prc`, with default values `em.tol` $= 10^{-6}$, and both `min.det` and `min.prc` with default value equal to the smallest positive floating point number representable on the computer (that is $2.225074\times10^{-308}$ for the R package used to code the numerical experiments in this paper). For any given $\delta, \pi_{\max}, \gamma$ define an initial choice of $\theta^{(0)} \in \Theta$. Let $s = 0, 1, 2, \ldots$ be the iteration index of the algorithm, so that $\theta^{(s)}$ is the value of the parameter $\theta$ computed at the $s$th iteration. In each step of the EM-algorithm perform the following substeps (complexity is caused by the requirement to deal with a number of potential degeneracies):

1. compute $\tau_j(x_i; \theta^{(s)})$ for all $i = 1, 2, \ldots, n$ and $j = 1, 2, \ldots, G$ (these quantities are given as initial values for $s = 0$);
2. if for some $i = 1, 2, \ldots, n$, $\tau_j(x_i, \theta^{(s)}) = 0$ (numerically) for all $j = 0, 1, \ldots, G$;
   - 2.a. if $\delta > 0$ set $\tau_0(x_i, \theta^{(s)}) \hookleftarrow 1$ and $\tau_j(x_i, \theta^{(s)}) \hookleftarrow 0$ for all $j = 1, 2, \ldots, G$;
   - 2.b. if $\delta = 0$ assign $x_i$ to the cluster $j*$ for which the Euclidean distance to its center is minimized, then set $\tau_{j*}(x_i, \theta^{(s)}) \hookleftarrow 1$ and $\tau_j(x_i, \theta^{(s)}) \hookleftarrow 0$ for all $j \neq j*$;
3. if for some $j \neq 0$, $\tau_j(x_i, \theta^{(s)}) = 0$ (numerically) for all $i = 1, 2, \ldots, n$, set $\theta^{em} \hookleftarrow \theta^{(s)}$ stop the algorithm and record a flag;
4. Compute

$$\pi_j^{(s+1)} = \frac{1}{n}\sum_{i=1}^{n} \tau_j(x_i, \theta^{(s)}) \qquad \text{for all } \; j = 0, 1, \ldots, G,$$

$$\mu_j^{(s+1)} = \frac{1}{n\pi_j^{(s)}}\sum_{i=1}^{n} \tau_j(x_i, \theta^{(s)})\, x_i \qquad \text{for all } \; j = 1, 2, \ldots, G,$$

$$\Sigma_j^{(s+1)} = \frac{1}{n\pi_j^{(s)}}\sum_{i=1}^{n} \tau_j(x_i, \theta^{(s)})\, (x_i - \mu_j^{(s+1)})(x_i - \mu_j^{(s+1)})' \quad \text{for all } \; j = 1, 2, \ldots, G.$$

5. if $\pi_0^{(s+1)} > \pi_{\max}$, set $\theta^{em} \hookleftarrow \theta^{(s)}$, stop the algorithm and record a flag;
6. if $\pi_j^{(s+1)} <$`min.prc`, set $\theta^{em} \hookleftarrow \theta^{(s)}$, stop the algorithm and record a flag;
7. For all $j = 1, 2, \ldots, G$ compute the spectral decomposition of $\Sigma_j^{(s+1)} = U_j^{(s+1)}\Lambda_j^{(s+1)}U_j^{(s+1)'}$, where $\Lambda_j^{(s+1)} = \text{diag}(\lambda_{1,j}^{(s+1)}, \ldots, \lambda_{p,j}^{(s+1)})$ is the diagonal matrix of eigenvalues of $\Sigma_j^{(s+1)}$,

and $U_j^{(s+1)}$ is the matrix of the normalized corresponding eigenvectors. If $\prod_{k=1}^{p} \lambda_{k,j}^{(s+1)} <$ `min.det`: find the smallest $\underline{k}$ such that there exists $\underline{\lambda}$ for which $\underline{\lambda}^{\underline{k}} \prod_{h=\underline{k}+1}^{p} \lambda_{h,j}^{(s)} =$ `min.det`, and set $\lambda_{k,j}^{(s+1)} \hookleftarrow \underline{\lambda}$ for all $k = 1, 2, \ldots, \underline{k}$. Correct the covariance matrix by setting

$$\Sigma_j^{(s+1)} \hookleftarrow U_j^{(s+1)} \underline{\Lambda}_j^{(s+1)} U_j^{(s+1)'} \quad \text{with} \quad \underline{\Lambda}_j^{(s+1)} \hookleftarrow \operatorname{diag}\left(\underline{\lambda}, \ldots, \underline{\lambda}, \lambda_{\underline{k}+1,j}^{(s+1)}, \ldots, \lambda_{p,j}^{(s+1)}\right).$$

8. if $|l_n(\theta^{(s+1)}) - l_n(\theta^{(s)})| \leq$ `em.tol`:
   - 8.a. if $\lambda_{\max}(\theta^{(s+1)})/\lambda_{\min}(\theta^{(s+1)}) \leq \gamma$, set $\theta^{em} \hookleftarrow \theta^{(s+1)}$;
   - 8.b. if $\lambda_{\max}(\theta^{(s+1)})/\lambda_{\min}(\theta^{(s+1)}) > \gamma$, set $\lambda_{jk}^{em} \hookleftarrow \max\{\lambda_{jk}^{(s+1)}, \lambda_{\max}(\theta^{(s+1)})/\gamma\}$; for all $j = 1, 2, \ldots, G$ and $k = 1, 2, \ldots, p$. Then adjust the corresponding eigenvalue matrices setting $\Sigma_j^{em} \hookleftarrow U_j^{(s+1)} \Lambda_j^{em} U_j^{(s+1)'}$, and record a flag.
   - 8.c. stop iterating and return $\theta^{em}$

## 2.2 OTRIMLE numerical approximation

Fix $\beta$ and the following additional computing parameters: `lower.icd`, `upper.icd`, `opt.selector`. Solve the program (3.12) by "golden section search algorithm" (GSSA) of Kiefer (1953) over the candidate set $\{0\} \cup$[`lower.icd, upper.icd`]. Each step of the golden search requires a RIMLE evaluation as described previously. In the standard GSSA the algorithm starts from a point within (`lower.icd`, `upper.icd`) computed using the "golden ratio". If a better candidate is available this can be given as an additional input. At each RIMLE evaluation, do the following:

1. If `opt.selector=TRUE` (default): discard all $\delta$ values for which the RIMLE computation ends with one or more flags. If all $\delta$ values are discarded set `opt.selector=FALSE` and find again an OTRIMLE solution.
2. if `opt.selector=FALSE`: only discard $\delta$ values for which the RIMLE computation ends with an error flag related to $\pi_{\max}$ (the previous substep 5).

The OTRIMLE could be based on evaluating the RIMLE on a grid of $\delta$ values. We found that the GSSA increases efficiency by a big margin. In most numerical experiments we found that no more than 30 RIMLE evaluations are required even for extremely small `lower.icd` and large `upper.icd`. Notice that the GSSA only requires that the target function has at least a local minimum in the search domain. The golden search is performed over the interval [`lower.icd, upper.icd`], and then the solution is compared with the RIMLE at $\delta = 0$. This is because we always check against the solution without the noise component. One could set `lower.icd`=0, but there is a limit in approximating positive real numbers on a computer. For high dimensional problems, where density values are often extremely small, and there could still be a difference between $\theta_n(0)$ and $\theta_n(\varepsilon)$, where $\varepsilon$ is the smallest positive number representable on a computer. The constraint implementation and the use of `opt.selector` in the OTRIMLE will be explained in detail below.

**Remark 1.** There is an intimate connection between $\delta, \gamma, \pi_{\max}$. When $\delta$ is too large it happens that too many points are assigned to the noise component. This will drain points away from Gaussians, which may cause small eigenvalues for them. For a given $\gamma$, $\pi_{\max}$ there will be $\delta_{\max}$ such that for $\delta > \delta_{\max}$ the RIMLE solution is on the border of the parameter space. Fixed $\gamma$ and $\pi_{\max}$, such a $\delta_{\max}$ depends on the $P$ that generates data, and this is unknown. So when $\pi_{0,n}$ is near $\pi_{\max}$, and/or $\lambda_{\min}(\theta_n(\delta))$ is near 0, this is an indication that $\delta$ is approaching $\delta_{\max}$. This

means that for a given pair $(\gamma, \pi_{\max})$ there will be values of $\delta$ producing RIMLE solutions in the interior of $\Theta$, and $\delta$ values producing RIMLE solutions on the border. Moreover the smallest eigenvalue that makes the RIMLE well defined also depends on $\delta$.

The algorithm should be able to find small clusters with potentially small variance, and therefore we do not build the lower bound for the eigenvalues in the algorithm. Instead we avoid singularities by adjusting the minimum number of eigenvalues such that the determinant of the corresponding covariance matrix is positive at machine precision in any single EM step. The eigenratio constraint is then enforced only at the end of the EM run. This allows the algorithm to fully explore concentrated clusters. The parameter `min.prc` avoids RIMLE fits with fewer than $G$ components, because this would mean that the OTRIMLE target function is not always evaluated at versions of $\theta_n(\cdot)$ with $G$ mixture components.

The `opt.selector` switch has the role to discriminate between $\delta$ values that provide solutions on the border of the parameter space and $\delta$ values that provides solution in the interior. When `opt.selector=FALSE`, solutions violating the $\pi_{\max}$ condition are still discarded. This is because the violation of (3.7) is an indication that a too large $\delta$ has been explored. In other words $\pi_{\max}$ has two roles: (i) it makes the RIMLE functional well defined (together with the eigenratio constraint); (ii) from the practical viewpoint is is used to indirectly define the maximum level of the improper density. The default choice used in the main paper is to set `opt.selector=TRUE`. `opt.selector=FALSE` may be chosen if the researcher is interested in finding solutions on the border of the parameter space, which may particularly include very small (if not spurious) clusters with low within-cluster variation.

Regarding `opt.selector`, experience shows that within computation of the OTRIMLE at least if no random initializations are used, it is advantageous to discard $\delta$-values for which the RIMLE-solution ends up at the border of the parameter space (unless this happens for all $\delta$), enforcing (3.5), (3.6) or zero component proportions, because for these cases $D(\delta)$ may behave irregularly and the golden search may be led astray. This particularly rules out too large values of $\delta$, which will trigger (3.6). Experience shows that the set of values of discarded $\delta$-values is usually a single interval, often containing the largest values in the candidate set. Discarded solutions can be brought back if they are needed in later stages of the golden section search, which is not normally necessary.

## 2.3 Choice of initial values

Biernacki et al. (2003) and Karlis and Xekalaki (2003) studied the problem of initializing the EM for computing MLE of Gaussian mixtures models. Both works found that the EM solutions strongly depend on initial values. The EM convergence is rather slow, and often the EM approximates the best local maximum of the likelihood function in the proximity of the initial parameter values. One may assign the $n$ points to $G$ clusters at random and compute the EM solution for each of the many random initializations, and then one chooses the EM approximation with the largest likelihood. In this paper we are concerned with robustness. A small group of points not belonging to any Gaussian group may produce a bad local maximum in the objective function so that the EM doesn't move from the initials. So while many random initializations allow to explore different regions of the parameter space, in some data sets it is difficult to avoid random initialisations in which no cluster is contaminated in such a way that it leads to a bad local optimum. Furthermore when we compute the OTRIMLE, this is based on the RIMLE evaluation for several $\delta$ values. This means that the computational load implied by multiple random initials is multiplied by the number of $\delta$ values explored.

Instead of relying on random initials, we start partitioning the sample points into $G$ groups plus a noise component. Then cluster memberships are used to initialize the pseudo-posterior probabilities. The main issue during initialization is not to start with too small clusters. Therefore we consider as valid initial partitions only those containing at least `min.pr`$\times n$ observations in each group (the default is `min.pr`=0.005). Nearest neighbor based clutter/noise detection proposed by Byers and Raftery (1998) is applied to identify an initial set of noise points. The latter is implemented in the `NNclean` function in R's `prabclus` package by Hennig and Hausdorf (2015). Agglomerative hierarchical clustering based on ML criteria for Gaussian mixture models proposed by Banfield and Raftery (1993) is then used for finding initial Gaussian groups in the non-noise. This has been implemented in the `hc` function of R's `mclust` package by Fraley et al. (2012). The initialization consists of the following steps:

1. Perform `NNclean` to isolate points likely to belong to the noise component. Typically this step finds more noise than it is actually needed.
2. On the subset of non-noise points obtained from step 1, perform `hc` from the `mclust` package, allowing for unequal covariance matrices.
3. If the partition obtained in steps 1 and 2 is valid, go to the final step 8, otherwise continue with the following step.
4. Add the too small clusters identified in step 3 to the noise component; on the remaining points do step 2 again. If the partition is now valid go to the final step 8, otherwise continue with the following step.
5. Increment the noise component identified in step 4 by adding the too small clusters from step 4. On the remaining points perform the k-means partitioning with $G$ clusters with few random initializations. If the partition is now valid go to the final step 8, otherwise continue with the following step.
6. Add the too small clusters from step 5 to the noise component identified in 5. Repeat a maximum of 1000 random assignments and stop when the smallest cluster has at least `min.prc`$\times n$ points. For each random assignment, draw $G$ data points at random, cluster points around the $G$ random centers based on Euclidean distance minimization. If a valid partition is found, go to the final substep 8, otherwise continue with the following step.
7. If after 1000 random iteration in step 6 no valid partition has been obtained, return to the last (invalid) random partition and go to the final substep 8.
8. Set $\tau_j(x_i, \theta^{(0)}) = \mathbb{1}\{x_i \in j\text{th initial group}\}$ for $j = 1, 2, \ldots, G$, and $\tau_0(x_i, \theta^{(0)}) = \mathbb{1}\{x_i \in \text{initial noise component}\}$. Use the initial pseudo–posterior weights to initialize the RIMLE computation previously described.

The extensive simulation study discussed in Coretto and Hennig (2015), showed that this initialization performs much better than the random initialization. Usually steps 1–5 can produce sensible initial values even under the most adverse experimental design. We could hardly produce artificial data sets where steps 6–8 are needed in order to have an initial partition.

Note that rimle.o, rimle.op, tclust.o and tclust.op in the simulation study require to compute the RIMLE solution and the TCLUST solution for different values of $\delta$ and trimming level respectively. For a given dataset all RIMLE and TCLUST solutions are computed from the same starting partition as defined previously.

### 2.4 Computation of the MCD functional

This does not concern RIMLE and OTRIMLE computation, but the end of Section 4 of Coretto and Hennig (2015).

The vector of $\theta_C$ with cluster parameters is based on the MCD location and scatter computed at each $P_j$ in the DGP. When $P_j$ is the Gaussian distribution $m_j$ and $S_j$ coincide with the Gaussian expectation and covariance matrix. However, in the following simulation study deviations from Gaussianity are considered by exploring $P_j$ that are: (i) non-central multivariate Student-t distributed, (ii) non-central multivariate Student-t on some marginals and Gaussian on other marginals. In these cases, appropriate MCD parameters have to be derived to obtain the reference $\theta_C$. Although the required MCD parameters exist for the cases we will consider here (Cator and Lopuhaä, 2012), it is not easy to compute them in closed form. For non-Gaussian elements of the DGP we computed the MCD parameters by Monte Carlo integration based on $10^6$ random draws, assuming zero mean and unit scale matrix and using affine equivariance of the MCD for transformation, by the `cov.rob` function of the R package `MASS` (Venables and Ripley, 2002).

### 2.5 Additional remarks for the computation of misclassification rates

Given the size of the comparative simulation study, some precaution is taken dealing with situations where the algorithm fails to provide a clustering solution for numerical reasons. In each Monte Carlo replicate, given the initial clustering, the software goes trough the following steps:

1. A clustering method is applied. If a valid solution is available go to step 3, otherwise perform step 2.
2. The method is applied setting its iteration number limit equal to 1. If a solution is available go to step 3, otherwise set the corresponding misclassification rate equal to `NA` (i.e. not available).
3. Compute the misclassification rate using formula (4.2).

`NA` cases only happened in 11 replicates out of 1000 for ot.tclust.p when applied to Sunspot.1h, and for no other method. These cases have not been considered for computing Monte Carlo averages (and related standard errors). OTRIMLE based methods always provided a solution based on previous steps 1 and 3.

Note that for the majority of the Monte Carlo replicates initialization was successfully performed based on steps 1–3 and 8 described in Section 2.3. The additional initialization step 4 was required for a minor fraction of replicates on few DGPs.

## 3 Definition of DGPs

The vector of $\theta_C$ with cluster parameters is based on the MCD location and scatter computed at each $P_j$ in the DGP scaled for consistency at Gaussian distributions. When $P_j$ is the Gaussian distribution $m_j$ and $P_j$ coincide with the expectation and covariance matrix under $P_j$. Apart

from the normal case, we considered situations where $P_j$ is: (i) non-central multivariate Student-t distributed, (ii) non-central multivariate Student-t on some marginals and normal on other marginals. When $P_j$ is not normal, appropriate MCD parameters have to be derived. Even though existence of the MCD parameters is guaranteed for a wide class of distributions (Cator and Lopuhaä, 2012), it is not easy to compute them in closed form solutions. For non-Gaussian elements of the DGP we computed the MCD parameters by Monte Carlo integration based on $10^6$ random draws. MCD has been computed with the `cov.rob` function of the `MASS` R package (Venables and Ripley, 2002).

For a covariance matrix $\Sigma$ define $Q(\Sigma) = U\sqrt{\Lambda}$, where $\sqrt{\Lambda}$ is the square root of the diagonal matrix of eigenvalues of $\Sigma$, and $U$ is the corresponding matrix of unit eigenvectors. Hence $\Sigma = Q(\Sigma)Q(\Sigma)'$. Let $\mathrm{N}(\mu, \Sigma)_p$ denote the $p$-dimensional Gaussian distribution with mean vector $\mu \in \mathbb{R}^p$ and $p \times p$ covariance matrix $\Sigma$. Let $t_v(\mu, \Sigma)_p$ be the $p$-dimensional non-central Student-t distribution with $v$ degrees of freedom, expectation $\mu$, and covariance matrix $\Sigma$. Notice that usually the non-central Student-t distribution is parametrized in terms of a scale matrix which is given by $(v-2)\Sigma/v$. Define $0_p$ as the $p$-dimensional zero vector, while $I_p$ is the usual $p \times p$ identity matrix. According to the notation in Coretto and Hennig (2015) we will make use of four types of cluster generating distributions $P_j$ for which MCD parameters are approximated as follows:

**Gaussian:** $P_j = \mathrm{N}(\mu_j, \Sigma_j)_p$. In this case $m_j = \mu_j$ and $S_j = \Sigma_j$.

**Student-t:** $P_j = \mathrm{t}_3(\mu_j, \Sigma_j)_2$. We computed the Monte Carlo approximation of the MCD center and scale for a $t_3(0_2, I_2)_2$. Let them be $m_{MC}$ and $S_{MC}$, respectively. Using the affine equivariance we define $m_j = \mu_j + Q(\Sigma_j)m_{MC}$ and $S_j = Q(\Sigma_j)S_{MC,1}Q(\Sigma_j)'$. This results in $m_{MC} = 0_2$, whereas $S_{MC}$ is diagonal matrix with $S_{MC}[k,k] = 0.3643$ for $k = 1, 2$.

**GaussT:** $P_j = \mathrm{GaussT}(\mu_j, \Sigma_j)$ is a 20-dimensional distribution with $\mathrm{N}(\mu_j, \Sigma_j)_2$ on the first two marginals and an independent $\mathrm{t}_3(0_{18}, I_{18})_{18}$ on the remaining marginals. Let $m_{MC}$ and $S_{MC}$ the Monte Carlo approximation of the MCD center and scale of a $\mathrm{GaussT}(0_{20}, I_{20})$ distribution. Let $\dot{\Sigma}_j$ be a $20 \times 20$ matrix obtained by replacing the elements of the block $\{I_{20}[r,c]\}_{r=1,2}^{c=1,2}$ with $\Sigma_j$; let $\dot{\mu}_j$ be the vector obtained by replacing the first two elements of $0_{20}$ with those of $\mu_j$. Using the affine equivariance we define $m_j = \dot{\mu}_j + Q(\dot{\Sigma}_j)m_{MC}$ and $S_j = Q(\dot{\Sigma}_j)S_{MC}Q(\dot{\Sigma}_j)'$. Here $m_{MC} = 0_{20}$ while $S_{MC}$ is diagonal matrix with $S_{MC}[k,k] = 0.9829$ for $k = 1, 2$, and $S_{MC}[k,k] = 0.3247$ for $k = 3, \ldots, 20$.

**TGauss:** $P_j = \mathrm{TGauss}(\mu_j, \Sigma_j)$ is 20-dimensional distribution with $\mathrm{t}_3(\mu_j, \Sigma_j)_2$ on the first two marginals, and an independent $\mathrm{N}(0_{18}, I_{18})_{18}$ on the remaining marginals. Let $m_{MC}$ and $S_{MC}$ be respectively Monte Carlo approximation of the MCD center and scale for a $\mathrm{TGauss}(0_{20}, I_{20})$ distribution. Let $\dot{\Sigma}_j$ be a $20 \times 20$ matrix obtained by replacing the elements of the block $\{I_{20}[r,c]\}_{r=1,2}^{c=1,2}$ with $\Sigma_j$; let $\dot{\mu}_j$ be the vector obtained by replacing the first two elements of $0_{20}$ with those of $\mu_j$. Using the affine equivariance we define $m_j = \dot{\mu}_j + Q(\dot{\Sigma}_j)m_{MC}$ and $S_j = Q(\dot{\Sigma}_j)S_{MC}Q(\dot{\Sigma}_j)'$. In this case $m_{MC} = 0_{20}$, whereas $S_{MC}$ is diagonal matrix with $S_{MC}[k,k] = 0.5023$ for $k = 1, 2$, and $S_{MC}[k,k] = 0.9739$ for $k = 3, \ldots, 20$.

Let $\mathrm{U}(a,b)$ with $a, b \in \mathbb{R}^2$ be the uniform distribution on the rectangle $[a_1, b_1] \times [a_2, b_2]$. Denote by $\mathrm{UGauss}(a,b)$ a 20-dimensional distribution that has a $\mathrm{Uniform}(a,b)$ on the first two marginals and an independent $\mathrm{N}(0_{18}, I_{18})_{18}$ on the remaining marginals. The 24 DGPs considered in the Monte Carlo comparison are defined as follows:

**WideNoise.2l** $G = 2$, $\pi_0 = 0.05$, $\pi_1 = 0.75$, $\pi_2 = 0.2$. $P_0 = \mathrm{U}(a, b)_2$ with $a = (-10, 10)'$ and $b = (-5, -15)'$. $P_j = \mathrm{N}(\mu_j, \Sigma_j)_2$ for $j = 1, 2$, where: $\mu_1 = (0, 5)'$, $\Sigma_1 = 0.2I_2$ $\mu_2 = (1, 5)'$, $\Sigma_2 = I_2$.

**WideNoise.2h** high dimensional version of WideNoise.2l with $P_0 = \mathrm{UGauss}(a, b)$ and $P_j = \mathrm{N}(\mu_j, \Sigma_j)_{20}$ for $j = 1, 2$. All parameters are the same as in WideNoise.2l except that now $\mu_{j,k} = 0$ and $\Sigma_j[k, k] = 1$ for $j = 1, 2$, and $k = 3, 4, \ldots, 20$, while $\Sigma_j[r, c] = 0$ for all $r \neq c$ with $r$ and $c$ taking values in $\{3, 4, \ldots, 20\}$.

**WideNoise.3l** $G = 3$, $\pi_0 = 0.1$, $\pi_j = 0.3$ for $j = 1, 2, 3$. $P_0 = \mathrm{U}(a, b)_2$ with $a = (-10, 10)'$ and $b = (-5, -15)'$. $P_j = \mathrm{N}(\mu_j, \Sigma_j)_2$ for $j = 1, 2, 3$, where: $\mu_1 = (0, 3)'$, $\Sigma_1[1, 1] = \Sigma_1[2, 2] = 1$, $\Sigma_1[1, 2] = 0.5$; $\mu_2 = (7, 1)'$, $\Sigma_2[1, 1] = \Sigma_2[2, 2] = 2$, $\Sigma_2[1, 2] = -1.5$ $\mu_3 = (5, 9)'$, $\Sigma_3[1, 1] = \Sigma_3[2, 2] = 2$, $\Sigma_3[1, 2] = 1.3$.

**WideNoise.3h** high dimensional version of WideNoise.3l with $P_0 = \mathrm{UGauss}(a, b)$ and $P_j = \mathrm{N}(\mu_j, \Sigma_j)_{20}$ for $j = 1, 2, 3$. All parameters are the same as in WideNoise.3l except that now $\mu_{j,k} = 0$ and $\Sigma_j[k, k] = 1$ for all $j = 1, 2, 3$ and $k = 3, 4, \ldots, 20$, while $\Sigma_j[r, c] = 0$ for all $r \neq c$ with $r$ and $c$ taking values in $\{3, 4, \ldots, 20\}$.

**SideNoise.2l** $G = 2$, $\pi_0 = 0.1$, $\pi_1 = 0.1$, $\pi_2 = 0.8$. $P_0 = \mathrm{U}(a, b)_2$ with $a = b = (-50, 5)'$. $P_j = \mathrm{N}(\mu_j, \Sigma_j)_2$ for $j = 1, 2$, where: $\mu_1 = (-10, 5)'$, $\Sigma_1 = 0.4I_2$ $\mu_2 = (3, 13)'$, $\Sigma_2[1, 1] = \Sigma_2[2, 2] = 1.5$, $\Sigma_2[1, 2] = -1.1$.

**SideNoise.2h** high dimensional version of SideNoise.2l with $P_0 = \mathrm{UGauss}(a, b)$ and $P_j = \mathrm{N}(\mu_j, \Sigma_j)_{20}$ for $j = 1, 2$. All parameters are the same as in SideNoise.2l except that now $\mu_{j,k} = 0$ and $\Sigma_j[k, k] = 1$ for $j = 1, 2$ and $k = 3, 4, \ldots, 20$, while $\Sigma_j[r, c] = 0$ for all $r \neq c$ with $r$ and $c$ taking values in $\{3, 4, \ldots, 20\}$.

**SideNoise.3l** $G = 3$, $\pi_0 = 0.1$, $\pi_1 = 0.15, \pi_2 = 0.35, \pi_3 = 0.4$. $P_0 = \mathrm{U}(a, b)_2$ with $a = b = (-50, 5)'$. $P_j = \mathrm{N}(\mu_j, \Sigma_j)_2$ for $j = 1, 2, 3$, with parameters set as in WideNoise.3l except that $\mu_1 = 0_2$.

**SideNoise.3h** high dimensional version of SideNoise.3l. Again $P_0 = \mathrm{UGauss}(a, b)$ with $a = b = (-50, 5)'$, and $P_j = \mathrm{N}(\mu_j, \Sigma_j)_{20}$ for $j = 1, 2, 3$. All Gaussian parameters are the same as in WideNoise.3h except that now $\mu_{1,1} = \mu_{1,1} = 0$.

**SunSpot.3l** $G = 3$, $\pi_0 = 0.025$, $\pi_1 = 0.325$ for $j = 1, 2, 3$. $P_0 = \mathrm{U}(a, b)_2$ with $a = b = (10^5, 10^5 + 10)'$. $P_j = \mathrm{N}(\mu_j, \Sigma_j)_2$ for $j = 1, 2, 3$, with all Gaussian parameters set as in WideNoise.3l.

**SunSpot.3h** high dimensional version of SunSpot.3l. Proportion parameters and $a$ and $b$ set as SunSpot.3l, but $P_0 = \mathrm{UGauss}(a, b)_2$ while $P_j = \mathrm{N}(\mu_j, \Sigma_j)_{20}$ for $j = 1, 2, 3$ with all parameters set as in WideNoise.3h.

**SunSpot.5l** $G = 5$, $\pi_0 = 0.002$, $\pi_1 = \pi_4 = 0.1497$, $\pi_2 = \pi_5 = 0.2994$, $\pi_3 = 0.0998$. $P_0 = \mathrm{U}(a, b)_2$ with $a = b = (30, 40)'$ $P_j = \mathrm{N}(\mu_j, \Sigma_j)_2$ with $\mu_1, \mu_2, \mu_3, \Sigma_1, \Sigma_2, \Sigma_3$ set as in WideNoise.3l, $\mu_4 = (-11, 5)'$, $\Sigma_4 = 0.5I_2$, $\mu_5 = (-9, 5)'$, $\Sigma_5 = 2.5I_2$.

**SunSpot.5h** high dimensional version of SunSpot.5l with $P_0 = \mathrm{UGauss}(a, b)$ and $P_j = \mathrm{N}(\mu_j, \Sigma_j)_{20}$ for $j = 1, 2, 3, 4, 5$. All parameters are the same as in Sunspot.5l except that now $\mu_{j,k} = 0$ and $\Sigma_j[k, k] = 1$ for all $j = 1, 2, 3, 4, 5$ and $k = 3, 4, \ldots, 20$, while $\Sigma_j[r, c] = 0$ for all $r \neq c$ with $r$ and $c$ taking values in $\{3, 4, \ldots, 20\}$.

**TGauss.3l** $G = 3$, $\pi_0 = 0$, $\pi_j = 1/3$ for $j = 1, 2, 3$. $P_j = t_3(\mu_j; \Sigma_j)_2$ with $\mu_j$ and $\Sigma_j$ set as in WideNoise.3l for $j = 1, 2, 3$. Note that $\Sigma_j$ here denotes the covariance matrix of the multivariate non-central $t_3$-distribution.

**TGauss.3h** high dimensional version of TGauss.3l. Everything is set as in the low dimensional version except now that $P_j = \text{TGauss}(\mu_j; \Sigma_j)$ for $j = 1, 2, 3$.

**TGauss.5l** $G = 5$, $\pi_0 = 0$, $\pi_1 = \pi_4 = 0.15$, $\pi_2 = \pi_5 = 0.3$; $\pi_3 = 0.1$, $P_j = t_3(\mu_j; \Sigma_j)_2$ for all $j = 1, 2, \ldots, 5$, with all parameters set as in SunSpot.5l except that $\mu_4 = (-10, 5)'$, $\mu_5 = (3, 13)$, and $\Sigma_5 = 2.5 I_5$.

**TGauss.5h** high dimensional version of TGauss.5l. Everything is set as in the low dimensional version except now that $P_j = \text{TGauss}(\mu_j; \Sigma_j)$ for $j = 1, 2, \ldots, 5$.

**GaussT.2l** $G = 2$, $\pi_0 = 0$, $\pi_1 = 0.15$, $\pi_2 = 0.85$; $P_j = \text{N}(\mu_j; \Sigma_j)_2$ for $j = 1, 2$ with $\mu_1 = (-1, 0.5)'$ $\Sigma_1 = 0.2 I_2$, and $\mu_2 = (0.3, 1.3)'$ $\Sigma_2[1,1] = \Sigma_2[2,2] = 1; \Sigma_2[1,2] = -0.8$.

**GaussT.2h** high dimensional version of TGauss.2l. Everything is set as in the low dimensional version except now that $P_j = \text{GaussT}(\mu_j; \Sigma_j)$ for $j = 1, 2$.

**GaussT.3l** $G = 3$, $\pi_0 = 0$, $\pi_j = 1/3$ and $P_j = \text{N}(\mu_j; \Sigma_j)_2$ for $j = 1, 2, 3$ with pairs $(\mu_j; \Sigma_j)$ fixed as in WideNoise.3l.

**GaussT.3h** high dimensional version of GaussT.3l. Everything is set as in the low dimensional version except now that $P_j = \text{GaussT}(\mu_j; \Sigma_j)$ for $j = 1, 2, 3$.

**Noiseless.3l** $G = 3$, $\pi_0 = 0$, $\pi_j = 1/3$ and $P_j = N(\mu_j; \Sigma_j)_2$ with $\mu_j, \Sigma_j$ set as in WideNoise.3l for all $j = 1, 2, 3$.

**Noiseless.3h** high dimensional version of Noiseless.3l. Everything is set as in the low dimensional version except now that $P_j = \text{N}(\mu_j; \Sigma_j)_{20}$ with parameters set as in WideNoise.3h for all $j = 1, 2, 3$.

**Noiseless.5l** $G = 5$, expected proportions set as in TGauss.5l; $P_j = \text{N}(\mu_j; \Sigma_j)_2$ with all $\mu_j$ and $\Sigma_j$ parameters set as in TGauss.5l except that $\mu_j$ is divided by $\sqrt{3}$ for all $j = 1, 2, \ldots, 5$.

**Noiseless.5h** high dimensional version of Noiseless.5h. Difference with the lower dimensional version is that now $P_j = \text{N}(\mu_j; \Sigma_j)_{20}$ with $\mu_{j,k} = 0$ and $\Sigma_j[k,k] = 1$ for all $j = 1, 2, \ldots, 5$ while $\Sigma_j[c,r] = 0$ for all $r \neq c$ with the pair and $r, c$ taking values in $\{3, 4, \ldots, 20\}$.

For a design with $G$ clusters, a DGP produces $n$ points by sampling from distributions $P_1, P_2, \ldots, P_G$ so that an expected number of points $n\pi_j$ is sampled under $P_j$ for $j = 1, 2, \ldots, G$. For some designs noise is generated by adding a further component that is denoted by $P_0$. The expected proportion of points under $P_0$ is denoted by $\pi_0$. In each Monte Carlo replicate sampling is performed as follows: the vector $(n_0, n_1, \ldots, n_G)'$ is sampled from a Multinomial$(n, \pi_0, \pi_1, \ldots, \pi_G)$ distribution, then $n_j$ points are independently sampled from $P_j$ for all $j = 1, 2, \ldots, G$. Therefore, in each Monte Carlo sample is an i.i.d. sample from the mixture distribution $\pi_0 P_0 + \sum_{j=1}^{G} \pi_j P_j$.

# 4 Plots for the DGPs and misclassification rates from the simulation study

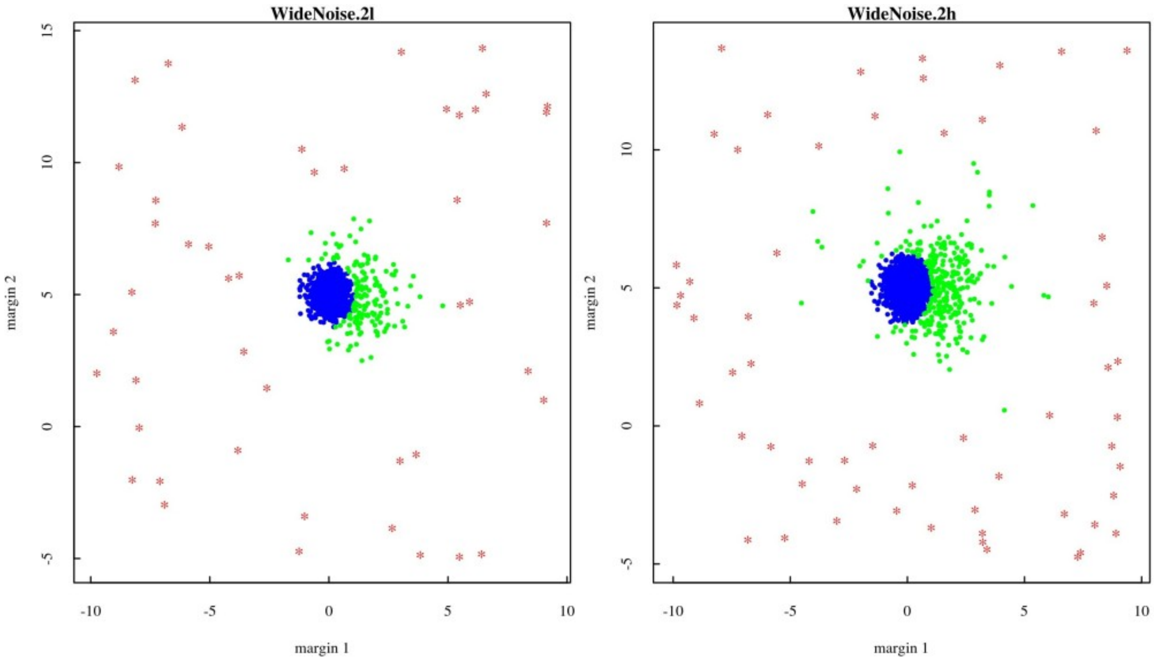


Figure 1: $\alpha$-Gaussian Regions for WideNoise.2 designs, with $\alpha = 10^{-4}$. Red stars are points defined as noise while clusters are denoted by colored points.

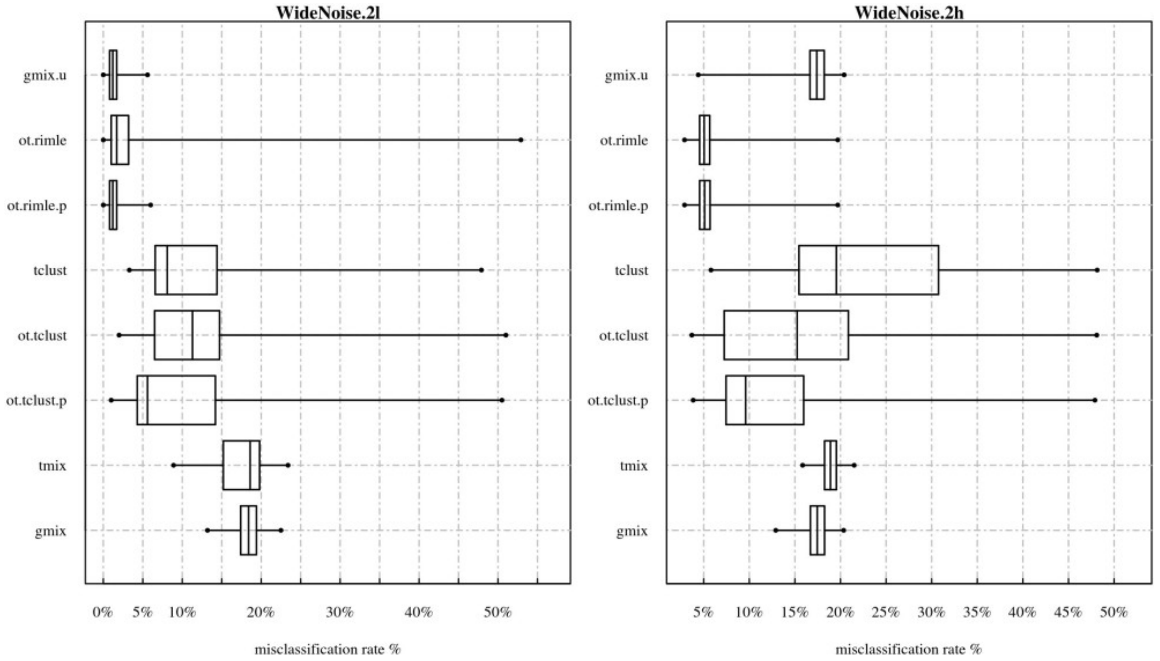


Figure 2: Boxplots for the Monte Carlo distribution of misclassification rates (%) for WideNoise.2 designs. Notice that the segment joining the whiskers' extremes always concides with the range of the distribution.

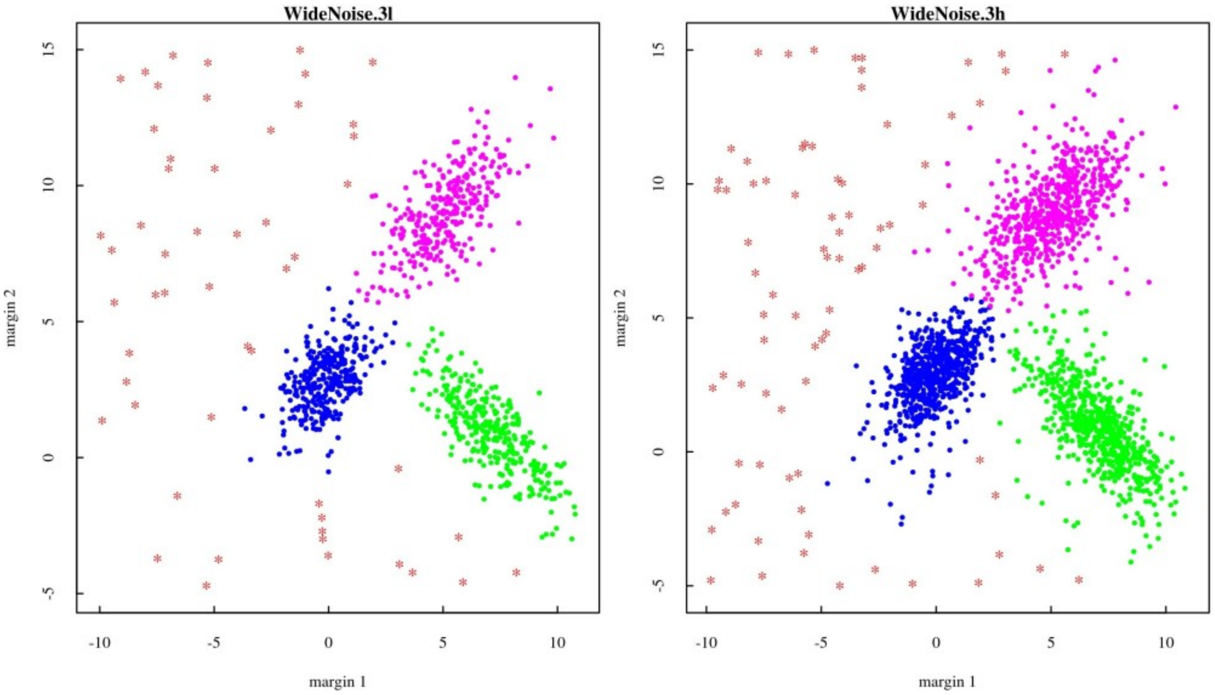


Figure 3: $\alpha$-Gaussian Regions for WideNoise.3 designs, with $\alpha = 10^{-4}$. Red stars are points defined as noise while clusters are denoted by colored points.

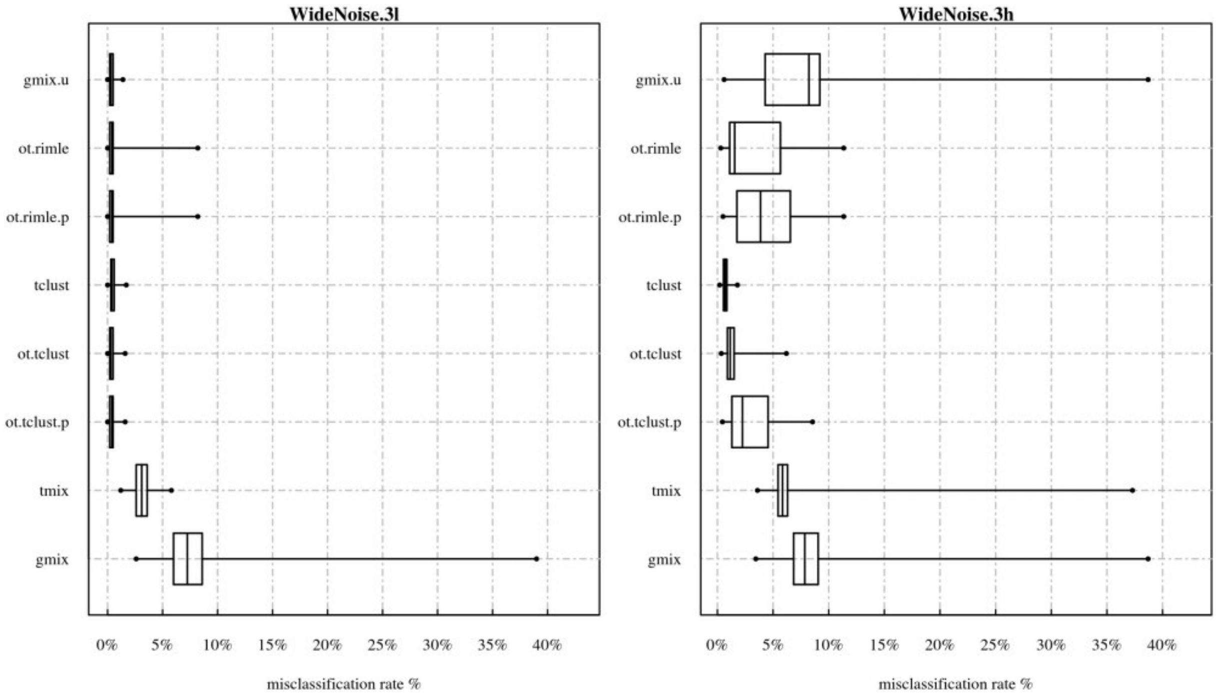


Figure 4: Boxplots for the Monte Carlo distribution of misclassification rates (%) for WideNoise.3 designs. Notice that the segment joining the whiskers' extremes always concides with the range of the distribution.

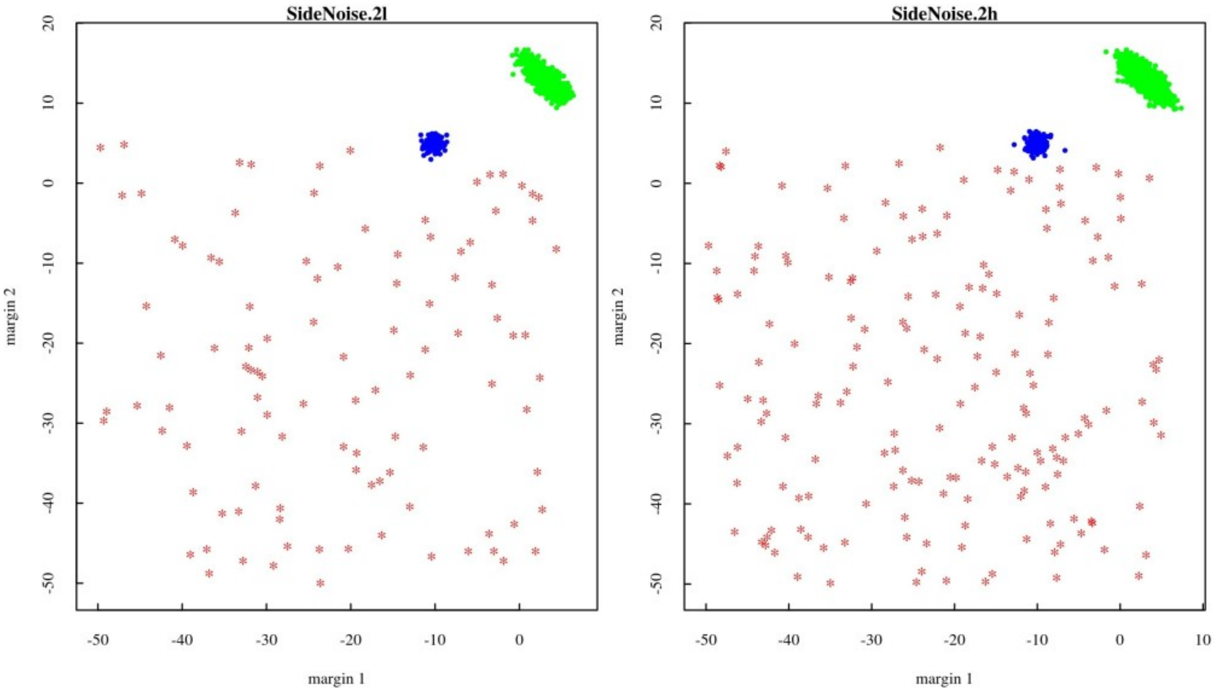


Figure 5: $\alpha$-Gaussian Regions for SideNoise.2 designs, with $\alpha = 10^{-4}$. Red stars are points defined as noise while clusters are denoted by colored points.

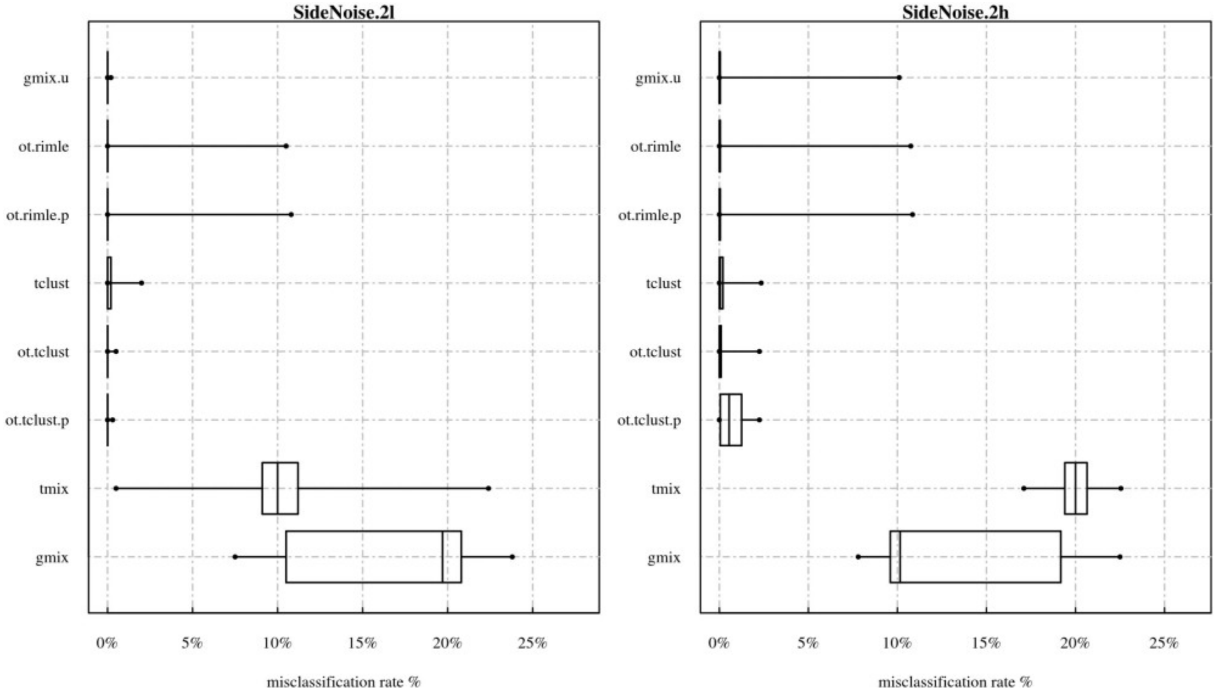


Figure 6: Boxplots for the Monte Carlo distribution of misclassification rates (%) for SideNoise.2 designs. Notice that the segment joining the whiskers' extremes always concides with the range of the distribution.

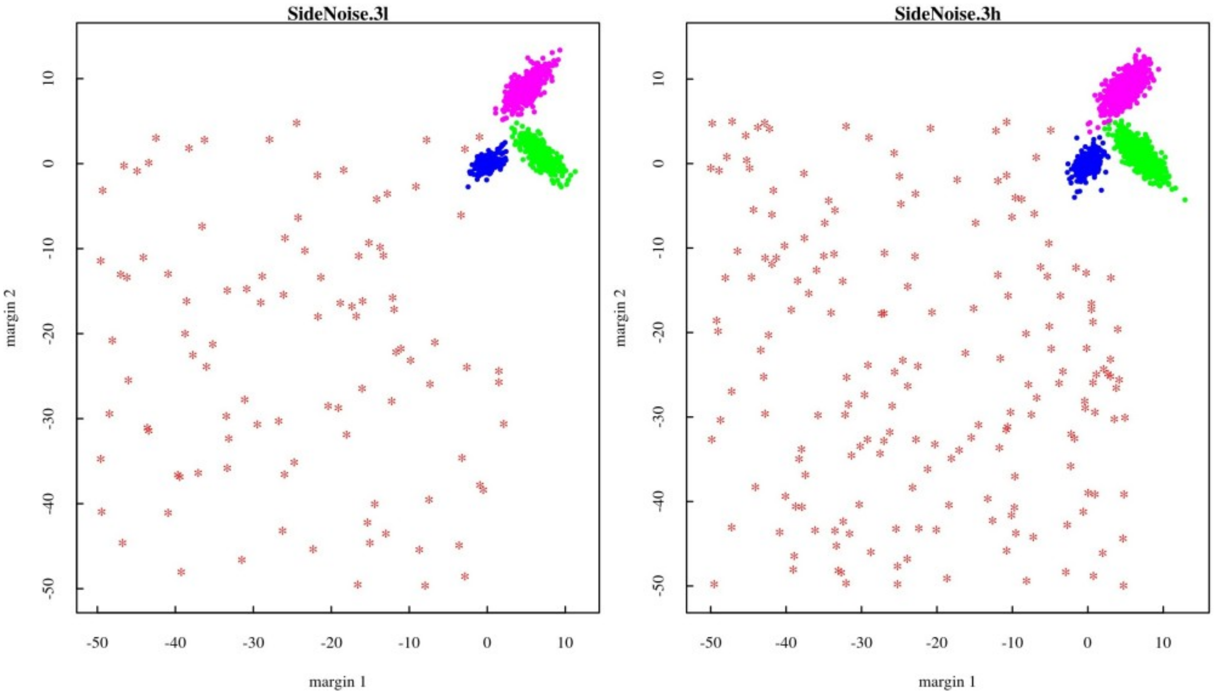


Figure 7: $\alpha$-Gaussian Regions for SideNoise.3 designs, with $\alpha = 10^{-4}$. Red stars are points defined as noise while clusters are denoted by colored points.

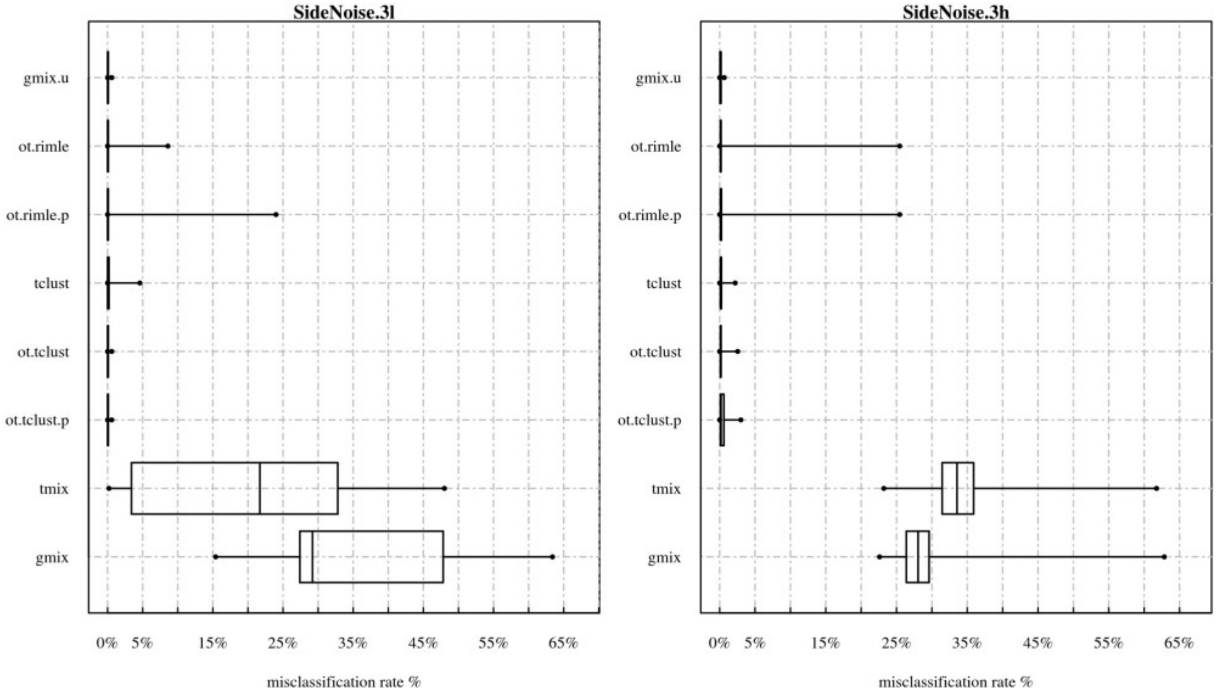


Figure 8: Boxplots for the Monte Carlo distribution of misclassification rates (%) for SideNoise.3 designs. Notice that the segment joining the whiskers' extremes always concides with the range of the distribution.

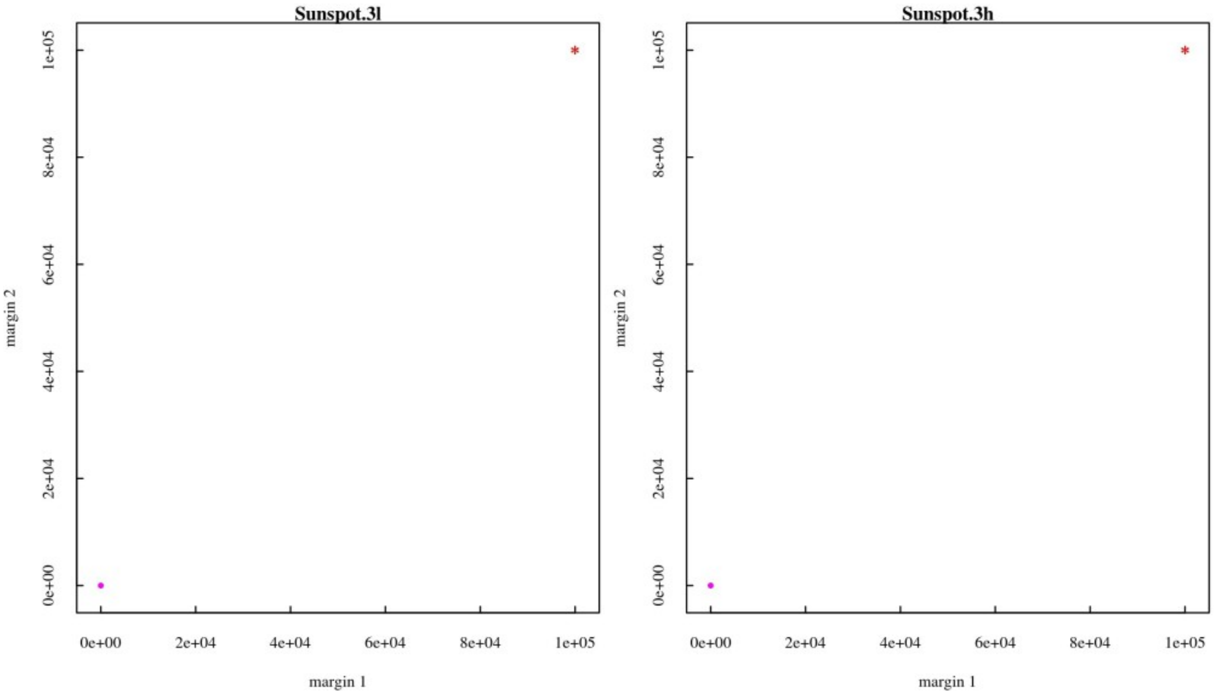


Figure 9: $\alpha$-Gaussian Regions for SunSpot.3 designs, with $\alpha = 10^{-4}$. Red stars are points defined as noise while clusters are denoted by colored points.

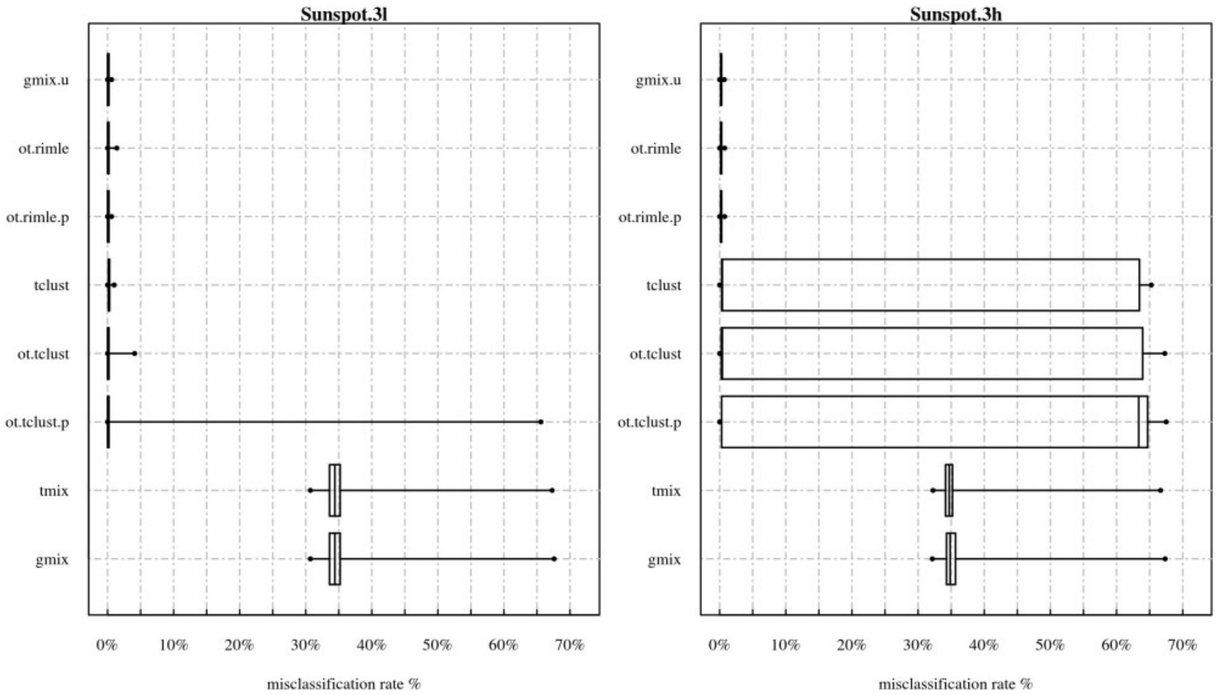


Figure 10: Boxplots for the Monte Carlo distribution of misclassification rates (%) for SunSpot.3 designs. Notice that the segment joining the whiskers' extremes always concides with the range of the distribution.

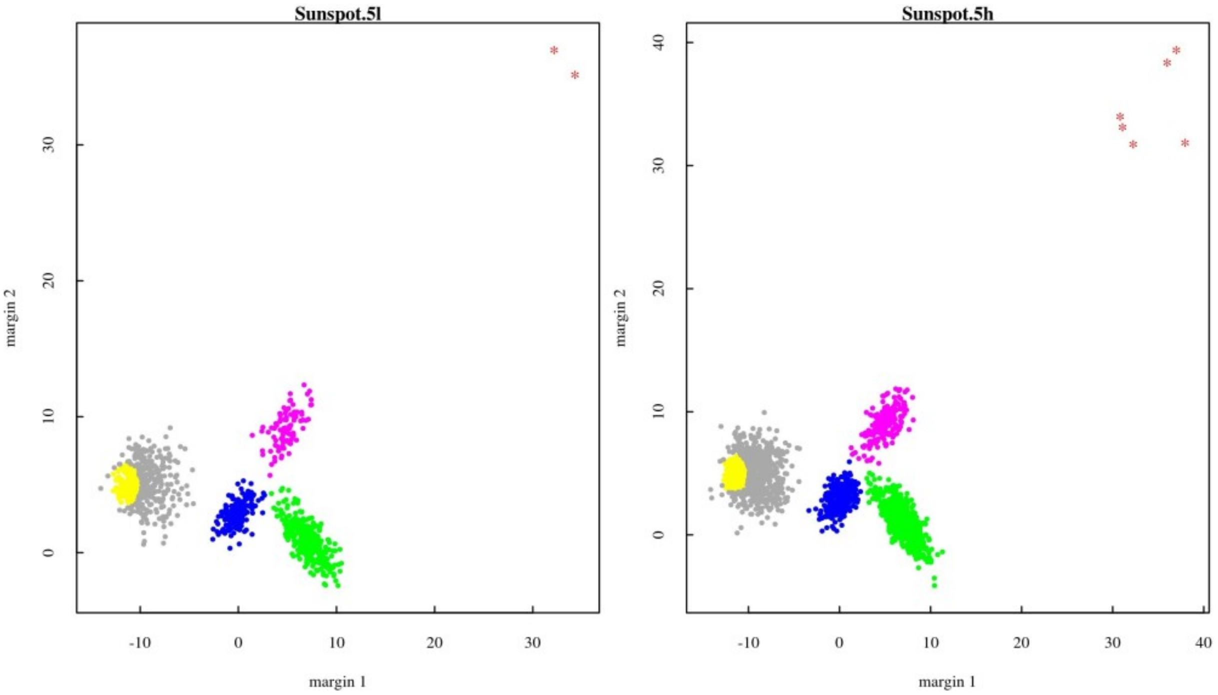


Figure 11: $\alpha$-Gaussian Regions for SunSpot.5 designs, with $\alpha = 10^{-4}$. Red stars are points defined as noise while clusters are denoted by colored points.

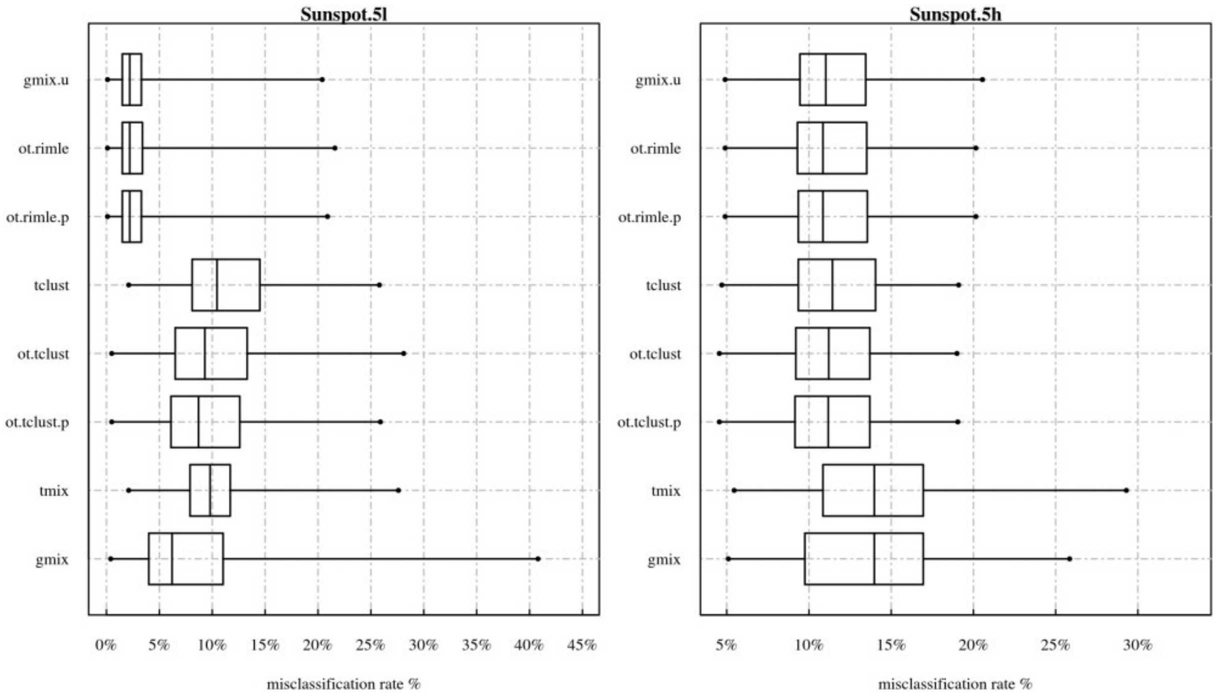


Figure 12: Boxplots for the Monte Carlo distribution of misclassification rates (%) for SunSpot.5 designs. Notice that the segment joining the whiskers' extremes always concides with the range of the distribution.

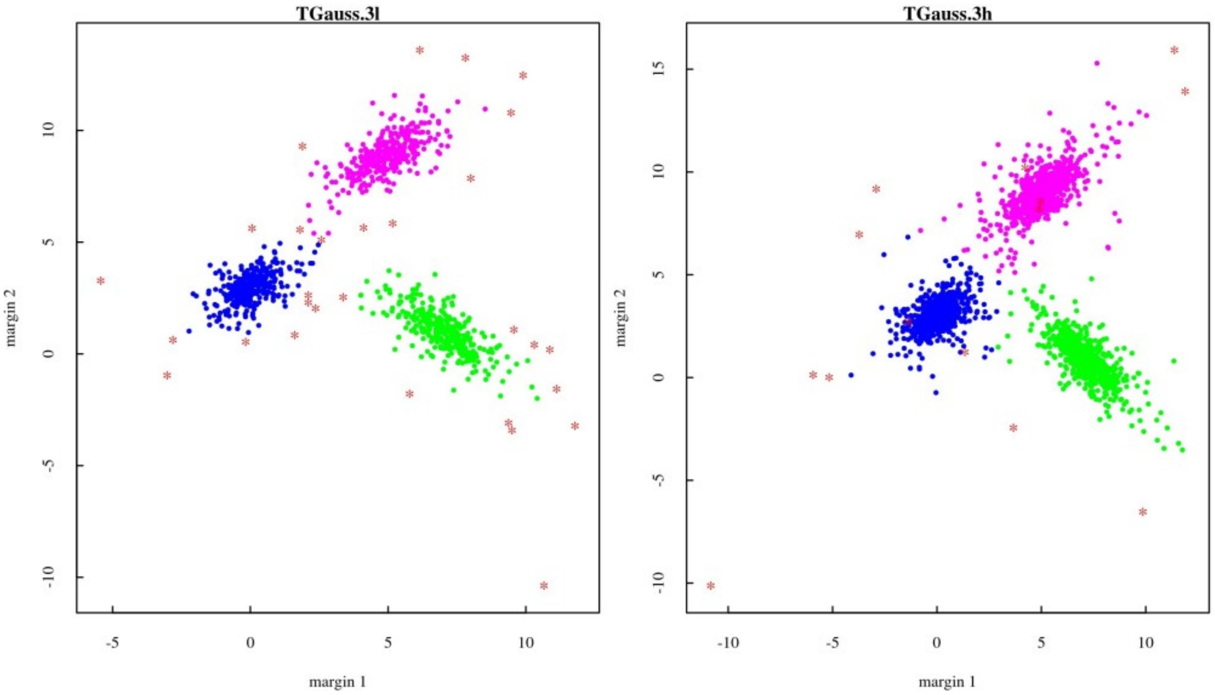


Figure 13: $\alpha$-Gaussian Regions for TGauss.3 designs, with $\alpha = 10^{-4}$. Red stars are points defined as noise while clusters are denoted by colored points.

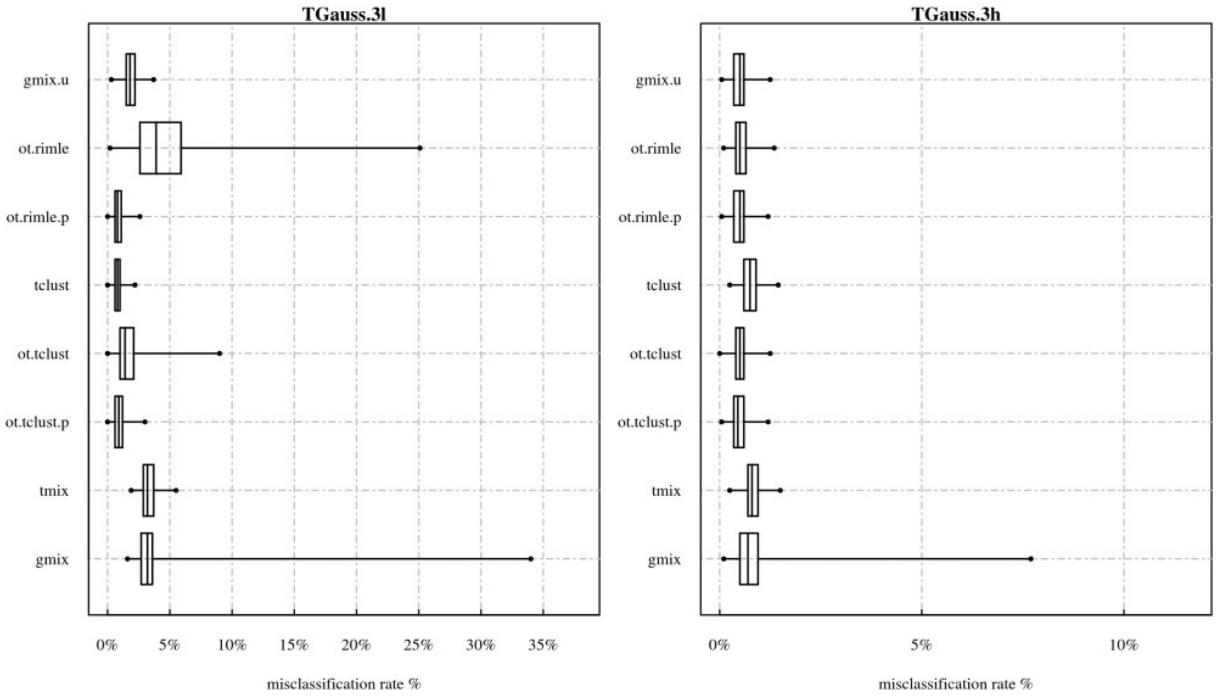


Figure 14: Boxplots for the Monte Carlo distribution of misclassification rates (%) for TGauss.3 designs. Notice that the segment joining the whiskers' extremes always concides with the range of the distribution.

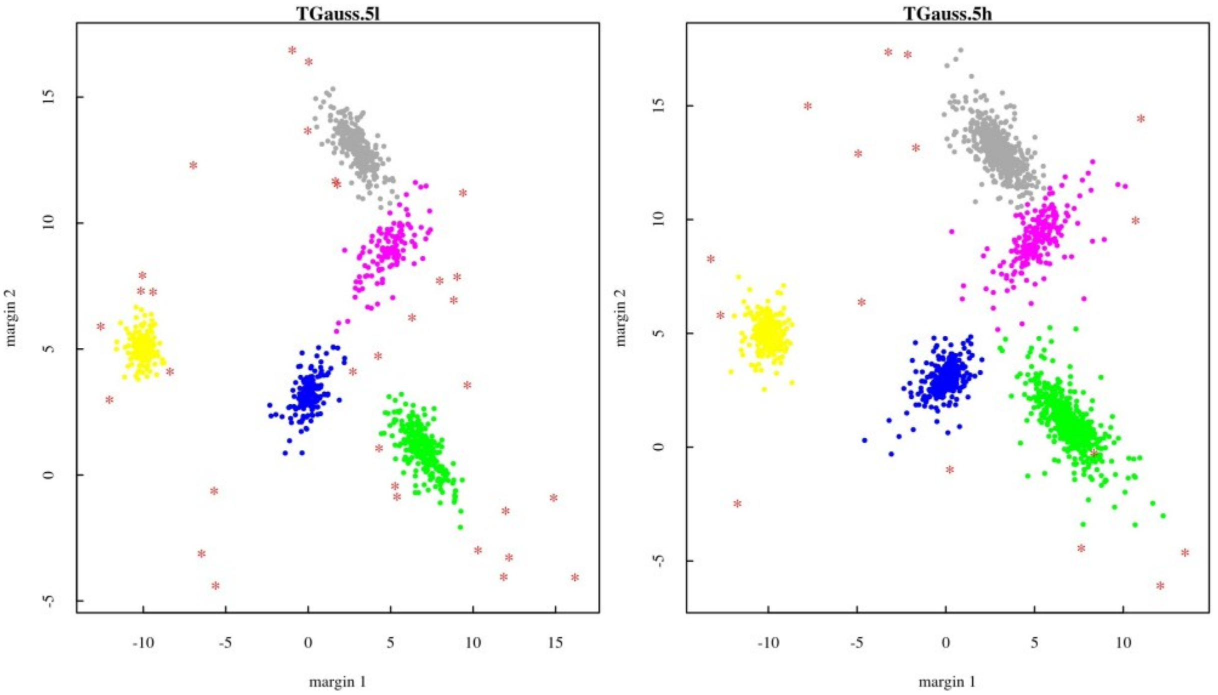


Figure 15: $\alpha$-Gaussian Regions for TGauss.5 designs, with $\alpha = 10^{-4}$. Red stars are points defined as noise while clusters are denoted by colored points.

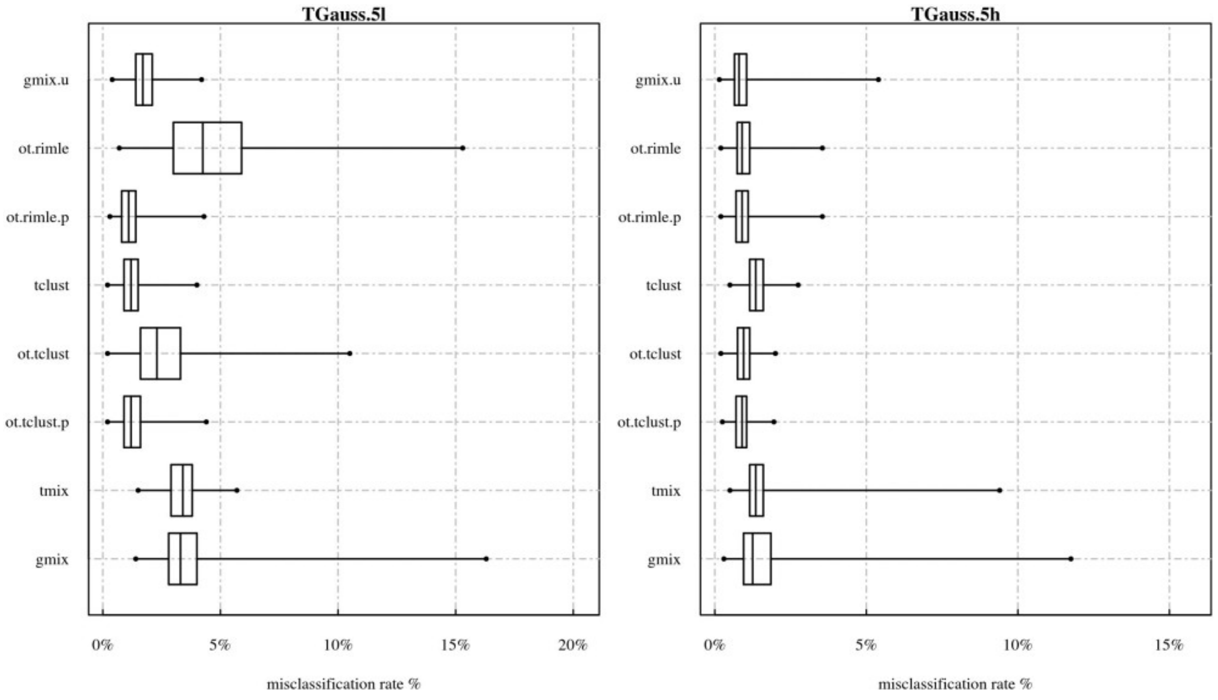


Figure 16: Boxplots for the Monte Carlo distribution of misclassification rates (%) for TGauss.5 designs. Notice that the segment joining the whiskers' extremes always concides with the range of the distribution.

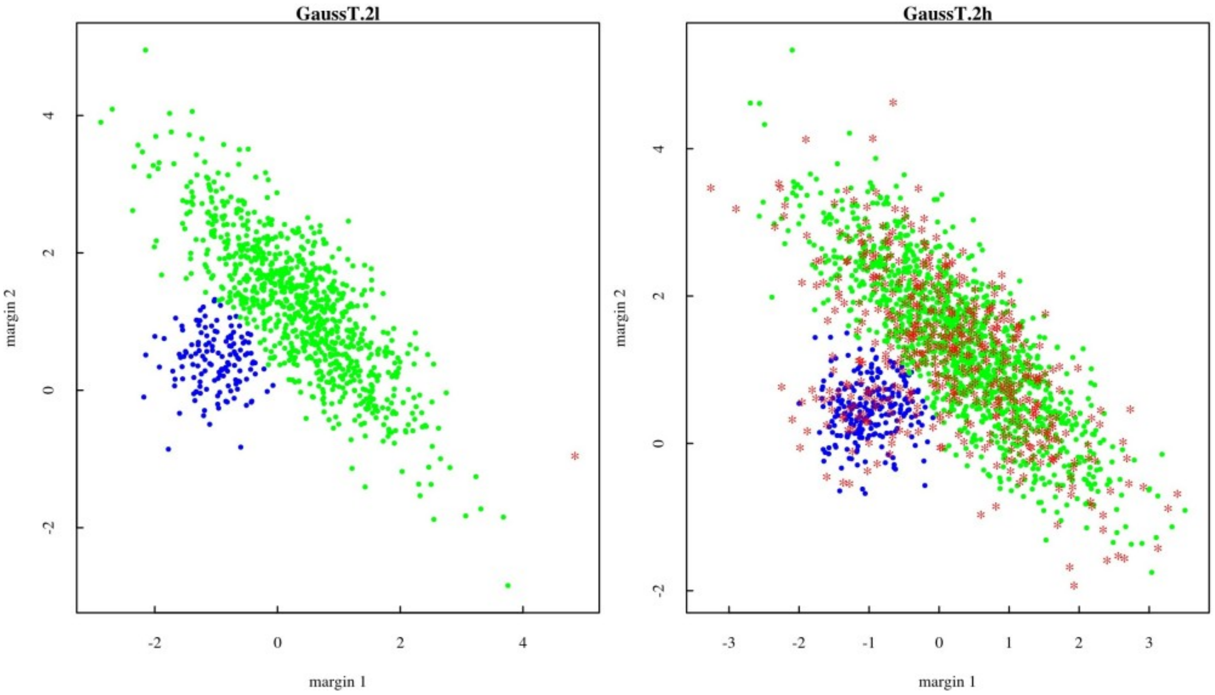


Figure 17: $\alpha$-Gaussian Regions for GaussT.2 designs, with $\alpha = 10^{-4}$. Red stars are points defined as noise while clusters are denoted by colored points.

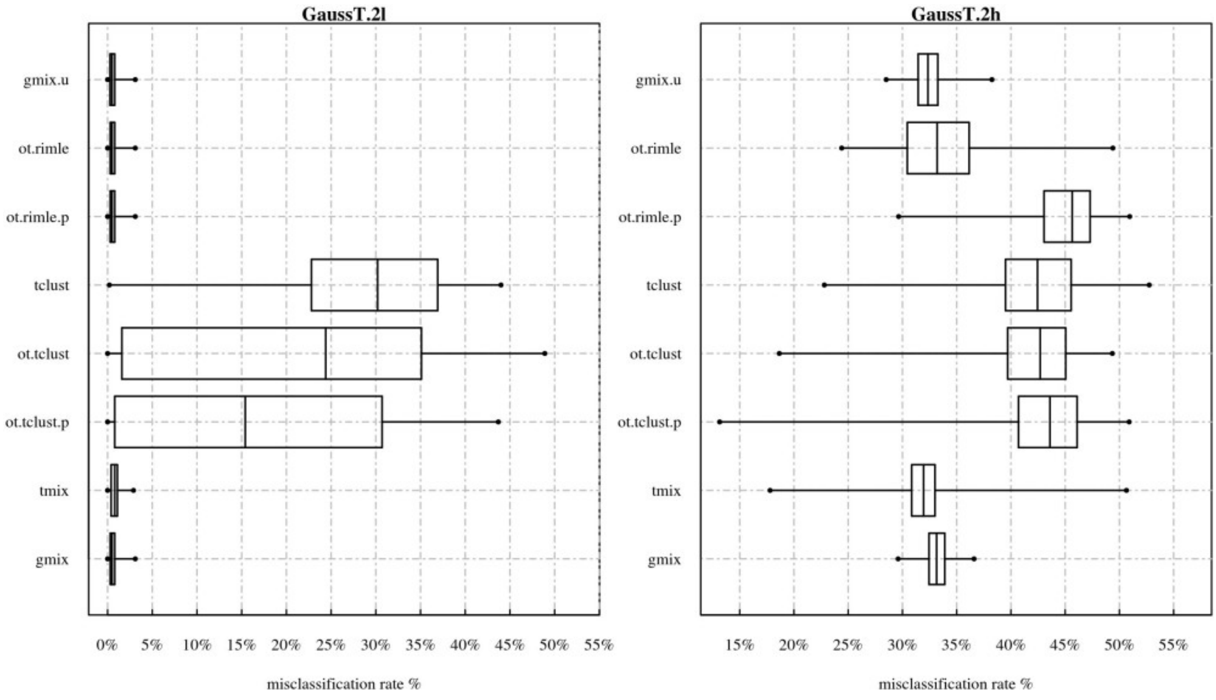


Figure 18: Boxplots for the Monte Carlo distribution of misclassification rates (%) for GaussT.2 designs. Notice that the segment joining the whiskers' extremes always concides with the range of the distribution.

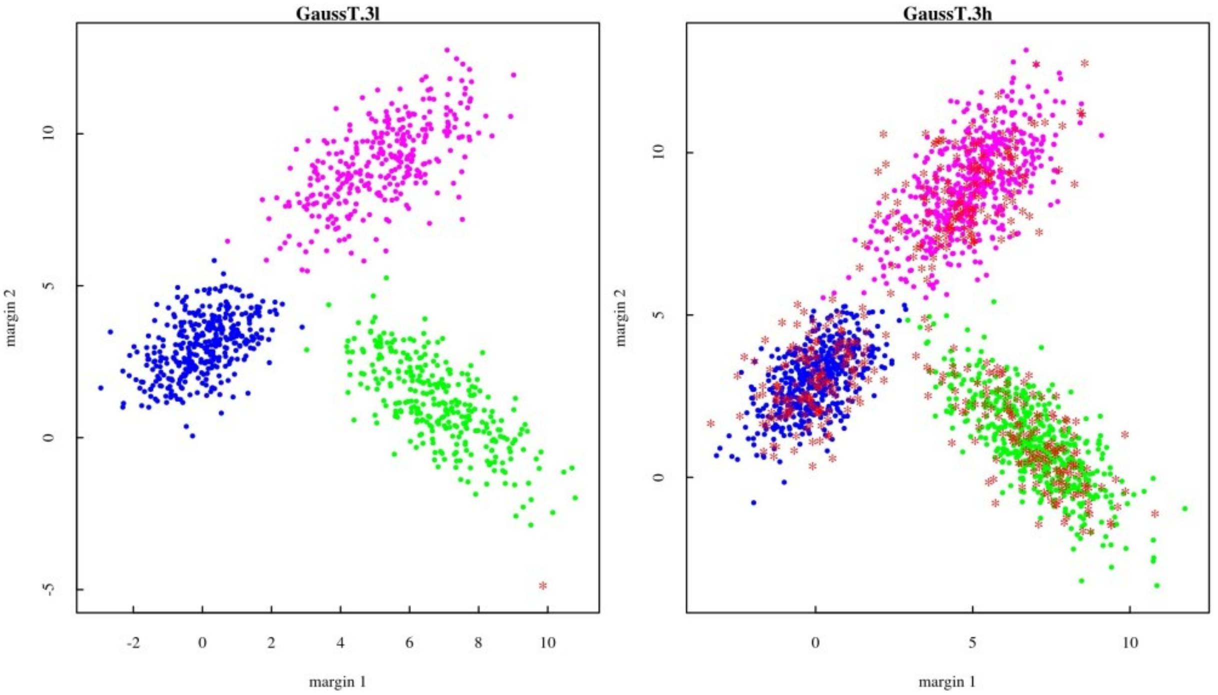


Figure 19: $\alpha$-Gaussian Regions for GaussT.3 designs, with $\alpha = 10^{-4}$. Red stars are points defined as noise while clusters are denoted by colored points.

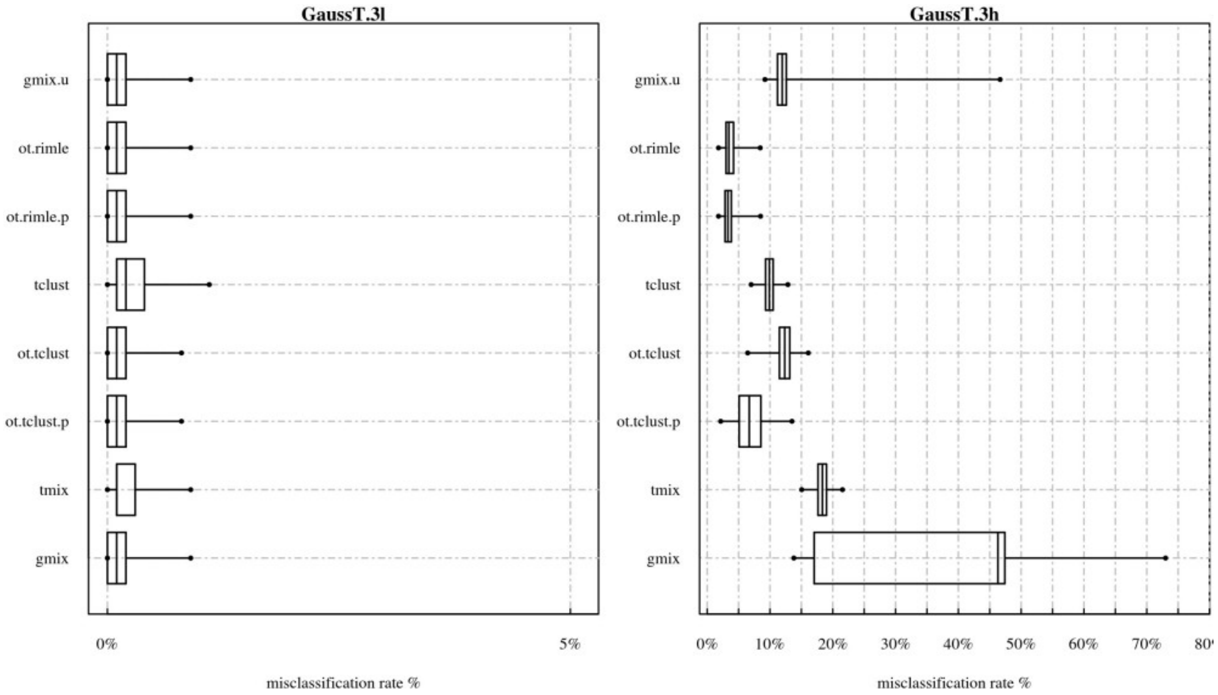


Figure 20: Boxplots for the Monte Carlo distribution of misclassification rates (%) for GaussT.3 designs. Notice that the segment joining the whiskers' extremes always concides with the range of the distribution.

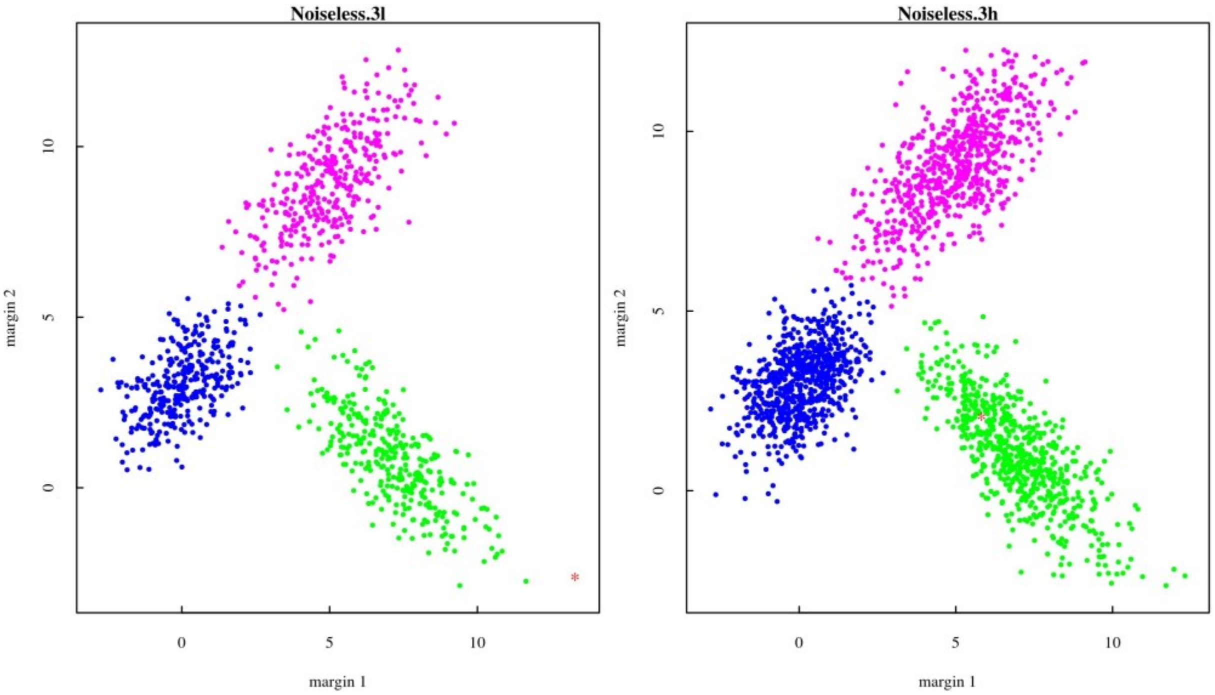


Figure 21: $\alpha$-Gaussian Regions for Noiseless.3 designs, with $\alpha = 10^{-4}$. Red stars are points defined as noise while clusters are denoted by colored points.

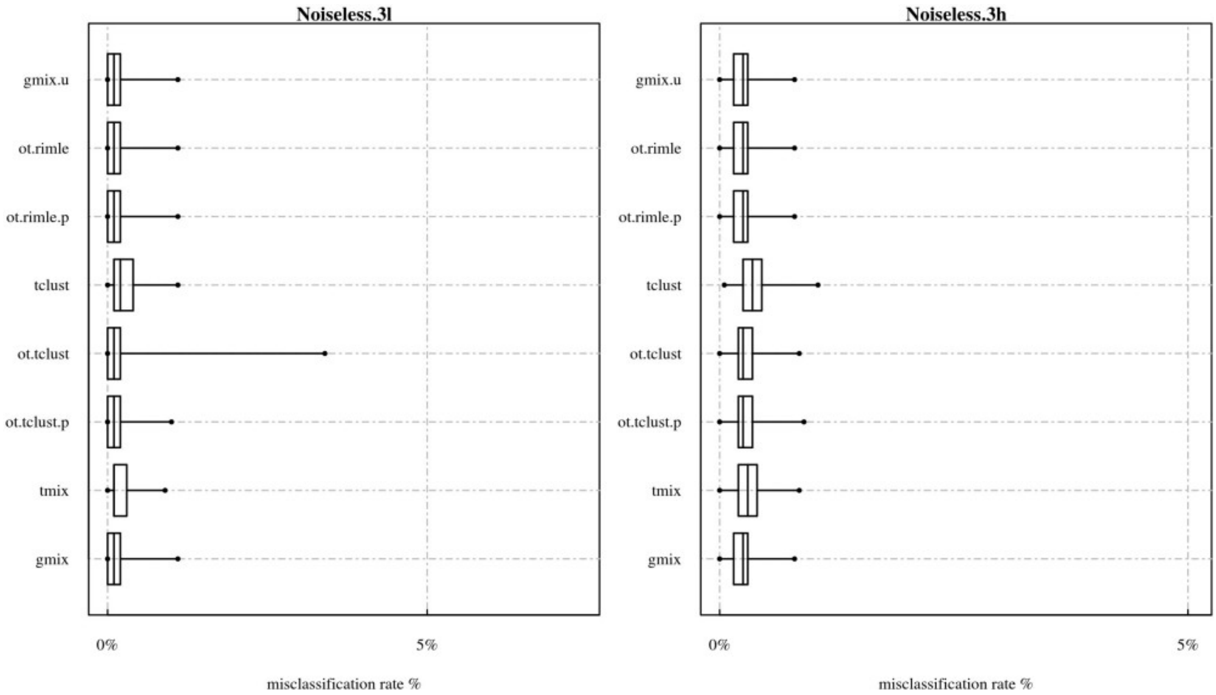


Figure 22: Boxplots for the Monte Carlo distribution of misclassification rates (%) for Noiseless.3 designs. Notice that the segment joining the whiskers' extremes always concides with the range of the distribution.

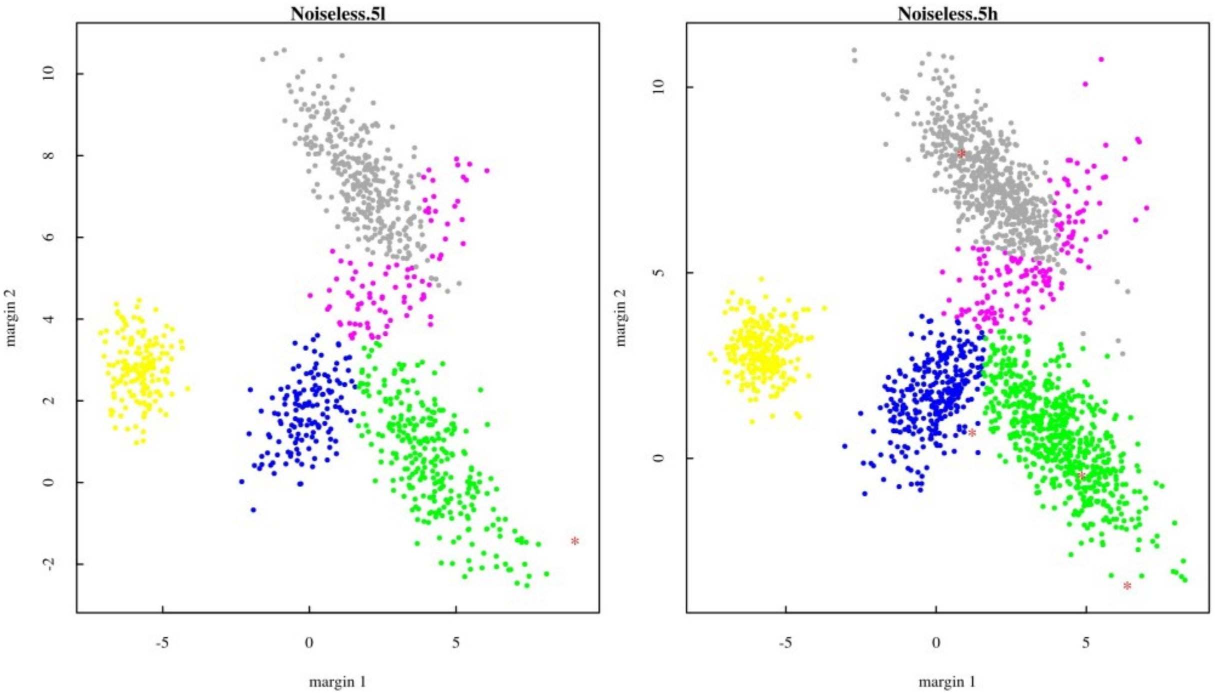


Figure 23: $\alpha$-Gaussian Regions for Noiseless.5 designs, with $\alpha = 10^{-4}$. Red stars are points defined as noise while clusters are denoted by colored points.

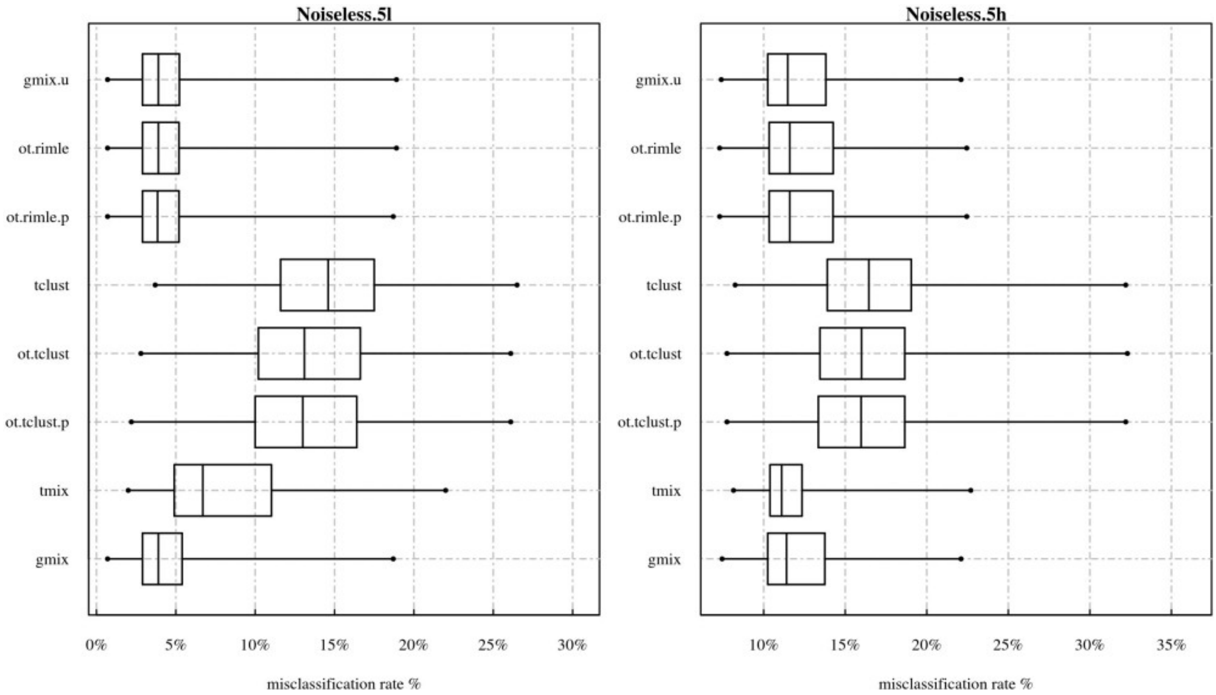


Figure 24: Boxplots for the Monte Carlo distribution of misclassification rates (%) for Noiseless.5 designs. Notice that the segment joining the whiskers' extremes always concides with the range of the distribution.

## 5 Detailed summary tables for the simulation study

Table 1: Monte Carlo estimates of the expected proportion of points belonging to noise region and the clusters. The index $j = 0$ denotes membership to the noise region, i.e. $\mathrm{NR}_\alpha$. Indexes $j = 1, 2, \ldots, 5$ denote $\alpha$-Gaussian regions. We set $\alpha = 10^{-4}$ for all designs. The table reports Monte Carlo averages and their standard errors multiplied by $10^4$ in brackets.

| DGP | Cluster Index | | | | | |
|---|---|---|---|---|---|---|
| | $j = 0$ | $j = 1$ | $j = 2$ | $j = 3$ | $j = 4$ | $j = 5$ |
| WideNoise.2l | 0.04(2.02) | 0.81(4.04) | 0.15(3.62) | — | — | — |
| WideNoise.2h | 0.04(1.31) | 0.81(2.86) | 0.16(2.60) | — | — | — |
| WideNoise.3l | 0.06(2.33) | 0.31(4.68) | 0.31(4.72) | 0.32(4.68) | — | — |
| WideNoise.3h | 0.05(1.50) | 0.32(3.24) | 0.32(3.34) | 0.32(3.35) | — | — |
| SideNoise.2l | 0.10(3.03) | 0.10(3.04) | 0.80(3.89) | — | — | — |
| SideNoise.2h | 0.10(2.08) | 0.10(2.18) | 0.80(2.84) | — | — | — |
| SideNoise.3l | 0.10(2.98) | 0.15(3.55) | 0.35(4.76) | 0.40(4.83) | — | — |
| SideNoise.3h | 0.10(2.06) | 0.15(2.65) | 0.35(3.36) | 0.40(3.56) | — | — |
| Sunspot.3l | 0.02(1.53) | 0.33(4.72) | 0.32(4.52) | 0.32(4.70) | — | — |
| Sunspot.3h | 0.03(1.10) | 0.33(3.26) | 0.32(3.35) | 0.32(3.19) | — | — |
| Sunspot.5l | 0.00(0.44) | 0.15(3.49) | 0.30(4.60) | 0.10(3.02) | 0.17(3.72) | 0.28(4.50) |
| Sunspot.5h | 0.00(0.32) | 0.15(2.53) | 0.30(3.24) | 0.10(2.04) | 0.17(2.56) | 0.28(3.21) |
| TGauss.3l | 0.04(1.99) | 0.32(4.64) | 0.32(4.48) | 0.32(4.78) | — | — |
| TGauss.3h | 0.01(0.57) | 0.33(3.32) | 0.33(3.25) | 0.33(3.32) | — | — |
| TGauss.5l | 0.04(1.95) | 0.14(3.61) | 0.29(4.64) | 0.10(3.03) | 0.14(3.51) | 0.28(4.42) |
| TGauss.5h | 0.01(0.58) | 0.15(2.52) | 0.30(3.23) | 0.11(2.25) | 0.15(2.51) | 0.29(3.30) |
| GaussT.2l | 0.00(0.09) | 0.15(3.56) | 0.85(3.57) | — | — | — |
| GaussT.2h | 0.22(3.02) | 0.12(2.17) | 0.66(3.41) | — | — | — |
| GaussT.3l | 0.00(0.07) | 0.33(4.79) | 0.33(4.55) | 0.33(4.61) | — | — |
| GaussT.3h | 0.23(3.03) | 0.26(3.15) | 0.26(3.15) | 0.26(3.01) | — | — |
| Noiseless.3l | 0.00(0.00) | 0.33(4.65) | 0.33(4.54) | 0.33(4.72) | — | — |
| Noiseless.3h | 0.00(0.00) | 0.33(3.26) | 0.33(3.28) | 0.33(3.38) | — | — |
| Noiseless.5l | 0.00(0.00) | 0.16(3.74) | 0.30(4.68) | 0.09(2.82) | 0.15(3.60) | 0.31(4.77) |
| Noiseless.5h | 0.00(0.00) | 0.16(2.64) | 0.30(3.15) | 0.09(2.00) | 0.15(2.52) | 0.31(3.36) |

Table 2: Monte Carlo average "noise-to-cluster" misclassification rates (%) with their standard errors in brackets. The "noise-to-cluster" misclassification rate gives the proportion of points belonging to the noise region assigned to one of the Gaussian clusters. Notice that both averages and their standard errors are reported in percentage scale.

| DGP | Method | | | | | | | |
|---|---|---|---|---|---|---|---|---|
| | gmix.u | ot.rimle | ot.rimle.p | tclust | ot.tclust | ot.tclust.p | tmix | gmix |
| WideNoise.2l | 0.04(0.00) | 0.03(0.00) | 0.08(0.00) | 0.00(0.00) | 0.00(0.00) | 0.05(0.01) | 3.93(0.04) | 4.28(0.02) |
| WideNoise.2h | 3.63(0.02) | 0.50(0.02) | 0.68(0.02) | 0.00(0.00) | 0.52(0.03) | 1.31(0.04) | 3.66(0.01) | 3.66(0.01) |
| WideNoise.3l | 0.09(0.00) | 0.11(0.01) | 0.21(0.01) | 0.04(0.00) | 0.14(0.00) | 0.18(0.01) | 2.77(0.02) | 5.02(0.04) |
| WideNoise.3h | 3.81(0.04) | 2.01(0.05) | 2.74(0.05) | 0.21(0.00) | 0.83(0.02) | 2.21(0.05) | 4.58(0.02) | 4.53(0.02) |
| SideNoise.2l | 0.00(0.00) | 0.02(0.01) | 0.04(0.02) | 0.17(0.01) | 0.00(0.00) | 0.01(0.00) | 9.58(0.05) | 10.00(0.03) |
| SideNoise.2h | 0.02(0.01) | 0.08(0.02) | 0.14(0.03) | 0.17(0.01) | 0.18(0.01) | 0.65(0.02) | 9.92(0.02) | 9.92(0.02) |
| SideNoise.3l | 0.01(0.00) | 0.01(0.00) | 0.03(0.01) | 0.10(0.01) | 0.01(0.00) | 0.01(0.00) | 6.73(0.12) | 9.82(0.03) |
| SideNoise.3h | 0.02(0.00) | 0.05(0.01) | 0.09(0.01) | 0.10(0.01) | 0.07(0.01) | 0.35(0.02) | 9.69(0.02) | 9.69(0.02) |
| Sunspot.3l | 0.00(0.00) | 0.00(0.00) | 0.00(0.00) | 0.00(0.00) | 0.00(0.00) | 0.03(0.01) | 2.49(0.02) | 2.49(0.02) |
| Sunspot.3h | 0.00(0.00) | 0.00(0.00) | 0.00(0.00) | 0.00(0.00) | 0.16(0.02) | 0.53(0.03) | 2.52(0.01) | 2.51(0.01) |
| Sunspot.5l | 0.00(0.00) | 0.00(0.00) | 0.00(0.00) | 0.00(0.00) | 0.00(0.00) | 0.00(0.00) | 0.01(0.00) | 0.02(0.00) |
| Sunspot.5h | 0.01(0.00) | 0.01(0.00) | 0.01(0.00) | 0.00(0.00) | 0.00(0.00) | 0.00(0.00) | 0.10(0.00) | 0.14(0.00) |
| TGauss.3l | 1.82(0.02) | 0.01(0.00) | 0.63(0.01) | 0.56(0.01) | 0.10(0.00) | 0.32(0.01) | 3.25(0.02) | 3.08(0.02) |
| TGauss.3h | 0.19(0.00) | 0.10(0.00) | 0.14(0.00) | 0.04(0.00) | 0.09(0.00) | 0.11(0.00) | 0.60(0.01) | 0.32(0.00) |
| TGauss.5l | 1.59(0.02) | 0.10(0.02) | 0.81(0.02) | 0.50(0.01) | 0.10(0.00) | 0.45(0.01) | 3.05(0.02) | 3.00(0.02) |
| TGauss.5h | 0.18(0.00) | 0.12(0.00) | 0.17(0.00) | 0.03(0.00) | 0.07(0.00) | 0.10(0.00) | 0.60(0.01) | 0.38(0.01) |
| GaussT.2l | 0.00(0.00) | 0.00(0.00) | 0.00(0.00) | 0.00(0.00) | 0.00(0.00) | 0.00(0.00) | 0.01(0.00) | 0.00(0.00) |
| GaussT.2h | 19.39(0.03) | 5.11(0.06) | 11.45(0.08) | 14.93(0.04) | 10.15(0.09) | 12.16(0.07) | 19.74(0.05) | 21.26(0.03) |
| GaussT.3l | 0.00(0.00) | 0.00(0.00) | 0.00(0.00) | 0.00(0.00) | 0.00(0.00) | 0.00(0.00) | 0.00(0.00) | 0.00(0.00) |
| GaussT.3h | 11.64(0.04) | 1.00(0.03) | 1.28(0.03) | 9.47(0.03) | 0.05(0.00) | 0.30(0.01) | 17.86(0.03) | 19.63(0.09) |
| Noiseless.3l | 0.00(0.00) | 0.00(0.00) | 0.00(0.00) | 0.00(0.00) | 0.00(0.00) | 0.00(0.00) | 0.00(0.00) | 0.00(0.00) |
| Noiseless.3h | 0.00(0.00) | 0.00(0.00) | 0.00(0.00) | 0.00(0.00) | 0.00(0.00) | 0.00(0.00) | 0.00(0.00) | 0.00(0.00) |
| Noiseless.5l | 0.00(0.00) | 0.00(0.00) | 0.00(0.00) | 0.00(0.00) | 0.00(0.00) | 0.00(0.00) | 0.00(0.00) | 0.00(0.00) |
| Noiseless.5h | 0.00(0.00) | 0.00(0.00) | 0.00(0.00) | 0.00(0.00) | 0.00(0.00) | 0.00(0.00) | 0.00(0.00) | 0.00(0.00) |

Table 3: Monte Carlo average “cluster-to-noise” misclassification rates (%) with their standard errors in brackets. The “cluster-to-noise” misclassification rate gives the proportion of points belonging to Gaussian clusters assigned to the noise component. Notice that both averages and their standard errors are reported in percentage scale.

| DGP | Method | | | | | | | |
|---|---|---|---|---|---|---|---|---|
| | gmix.u | ot.rimle | ot.rimle.p | tclust | ot.tclust | ot.tclust.p | tmix | gmix |
| WideNoise.2l | 0.06(0.00) | 1.01(0.07) | 0.03(0.00) | 2.55(0.03) | 4.07(0.07) | 2.23(0.08) | 0.00(0.00) | 0.00(0.00) |
| WideNoise.2h | 0.00(0.00) | 0.07(0.00) | 0.05(0.00) | 1.08(0.01) | 0.58(0.01) | 0.35(0.01) | 0.00(0.00) | 0.00(0.00) |
| WideNoise.3l | 0.11(0.00) | 0.17(0.01) | 0.04(0.00) | 0.24(0.01) | 0.09(0.00) | 0.06(0.00) | 0.00(0.00) | 0.00(0.00) |
| WideNoise.3h | 0.00(0.00) | 0.02(0.00) | 0.01(0.00) | 0.11(0.00) | 0.02(0.00) | 0.01(0.00) | 0.00(0.00) | 0.00(0.00) |
| SideNoise.2l | 0.01(0.00) | 0.01(0.00) | 0.01(0.00) | 0.01(0.00) | 0.01(0.00) | 0.01(0.00) | 0.00(0.00) | 0.00(0.00) |
| SideNoise.2h | 0.01(0.00) | 0.01(0.00) | 0.01(0.00) | 0.02(0.00) | 0.02(0.00) | 0.01(0.00) | 0.00(0.00) | 0.00(0.00) |
| SideNoise.3l | 0.01(0.00) | 0.03(0.01) | 0.01(0.00) | 0.01(0.00) | 0.02(0.00) | 0.01(0.00) | 0.00(0.00) | 0.00(0.00) |
| SideNoise.3h | 0.01(0.00) | 0.02(0.00) | 0.01(0.00) | 0.03(0.00) | 0.02(0.00) | 0.02(0.00) | 0.00(0.00) | 0.00(0.00) |
| Sunspot.3l | 0.00(0.00) | 0.01(0.00) | 0.00(0.00) | 0.07(0.00) | 0.01(0.00) | 0.00(0.00) | 0.00(0.00) | 0.00(0.00) |
| Sunspot.3h | 0.00(0.00) | 0.01(0.00) | 0.00(0.00) | 0.05(0.00) | 0.01(0.00) | 0.01(0.00) | 0.00(0.00) | 0.00(0.00) |
| Sunspot.5l | 0.02(0.01) | 0.03(0.01) | 0.01(0.01) | 0.68(0.01) | 0.27(0.02) | 0.10(0.01) | 0.00(0.00) | 0.00(0.00) |
| Sunspot.5h | 0.00(0.00) | 0.01(0.00) | 0.01(0.00) | 0.22(0.00) | 0.05(0.00) | 0.04(0.00) | 0.00(0.00) | 0.00(0.00) |
| TGauss.3l | 0.00(0.00) | 4.55(0.09) | 0.26(0.01) | 0.23(0.01) | 1.53(0.03) | 0.62(0.02) | 0.00(0.00) | 0.00(0.00) |
| TGauss.3h | 0.06(0.00) | 0.20(0.00) | 0.13(0.00) | 0.53(0.01) | 0.21(0.00) | 0.17(0.00) | 0.00(0.00) | 0.01(0.00) |
| TGauss.5l | 0.02(0.00) | 4.41(0.08) | 0.25(0.01) | 0.53(0.01) | 2.25(0.04) | 0.70(0.02) | 0.00(0.00) | 0.00(0.00) |
| TGauss.5h | 0.07(0.00) | 0.25(0.01) | 0.14(0.00) | 0.80(0.01) | 0.33(0.00) | 0.22(0.00) | 0.00(0.00) | 0.02(0.00) |
| GaussT.2l | 0.00(0.00) | 0.00(0.00) | 0.00(0.00) | 1.08(0.02) | 1.17(0.06) | 0.10(0.01) | 0.00(0.00) | 0.00(0.00) |
| GaussT.2h | 0.00(0.00) | 0.27(0.04) | 0.00(0.00) | 0.00(0.00) | 0.07(0.02) | 0.02(0.01) | 0.00(0.00) | 0.00(0.00) |
| GaussT.3l | 0.00(0.00) | 0.00(0.00) | 0.00(0.00) | 0.11(0.00) | 0.01(0.00) | 0.01(0.00) | 0.00(0.00) | 0.00(0.00) |
| GaussT.3h | 0.00(0.00) | 2.26(0.04) | 1.73(0.04) | 0.00(0.00) | 11.75(0.04) | 6.13(0.09) | 0.00(0.00) | 0.00(0.00) |
| Noiseless.3l | 0.01(0.00) | 0.01(0.00) | 0.01(0.00) | 0.11(0.00) | 0.02(0.00) | 0.01(0.00) | 0.00(0.00) | 0.01(0.00) |
| Noiseless.3h | 0.01(0.00) | 0.01(0.00) | 0.01(0.00) | 0.09(0.00) | 0.02(0.00) | 0.02(0.00) | 0.00(0.00) | 0.01(0.00) |
| Noiseless.5l | 0.02(0.00) | 0.01(0.00) | 0.01(0.00) | 0.63(0.01) | 0.20(0.01) | 0.12(0.00) | 0.00(0.00) | 0.01(0.00) |
| Noiseless.5h | 0.01(0.00) | 0.02(0.00) | 0.01(0.00) | 0.22(0.00) | 0.08(0.00) | 0.07(0.00) | 0.00(0.00) | 0.01(0.00) |

Table 4: Monte Carlo average "cluster-to-cluster" misclassification rates (%) with their standard errors in brackets. The "cluster-to-cluster" misclassification rate gives the proportion of points belonging to Gaussian clusters not assigned consistently to a Gaussian cluster. Notice that both averages and their standard errors are reported as percentages.

| DGP | Method | | | | | | | |
|---|---|---|---|---|---|---|---|---|
| | gmix.u | ot.rimle | ot.rimle.p | tclust | ot.tclust | ot.tclust.p | tmix | gmix |
| WideNoise.2l | 1.24(0.02) | 3.96(0.23) | 1.23(0.02) | 10.16(0.32) | 9.04(0.28) | 7.92(0.26) | 13.55(0.07) | 14.12(0.04) |
| WideNoise.2h | 13.72(0.04) | 4.71(0.04) | 4.67(0.05) | 21.85(0.32) | 15.10(0.33) | 11.20(0.26) | 15.24(0.03) | 13.77(0.03) |
| WideNoise.3l | 0.14(0.00) | 0.15(0.00) | 0.15(0.00) | 0.16(0.00) | 0.15(0.00) | 0.15(0.00) | 0.32(0.01) | 2.77(0.12) |
| WideNoise.3h | 3.78(0.16) | 1.15(0.04) | 1.52(0.04) | 0.40(0.01) | 0.46(0.01) | 0.82(0.02) | 1.32(0.03) | 4.02(0.14) |
| SideNoise.2l | 0.00(0.00) | 0.00(0.00) | 0.00(0.00) | 0.00(0.00) | 0.00(0.00) | 0.00(0.00) | 1.17(0.08) | 6.68(0.16) |
| SideNoise.2h | 0.00(0.00) | 0.00(0.00) | 0.00(0.00) | 0.00(0.00) | 0.00(0.00) | 0.00(0.00) | 10.11(0.02) | 2.69(0.15) |
| SideNoise.3l | 0.04(0.00) | 0.04(0.00) | 0.07(0.02) | 0.08(0.01) | 0.04(0.00) | 0.04(0.00) | 12.16(0.36) | 26.78(0.40) |
| SideNoise.3h | 0.09(0.00) | 0.12(0.02) | 0.14(0.02) | 0.12(0.00) | 0.11(0.00) | 0.16(0.00) | 24.53(0.16) | 21.89(0.31) |
| Sunspot.3l | 0.11(0.00) | 0.11(0.00) | 0.11(0.00) | 0.15(0.00) | 0.12(0.00) | 2.14(0.35) | 32.17(0.11) | 32.89(0.18) |
| Sunspot.3h | 0.23(0.00) | 0.23(0.00) | 0.23(0.00) | 21.33(0.95) | 27.02(0.99) | 36.29(1.00) | 32.23(0.06) | 37.49(0.37) |
| Sunspot.5l | 3.30(0.12) | 3.36(0.12) | 3.36(0.12) | 10.57(0.12) | 9.74(0.14) | 9.43(0.14) | 10.00(0.10) | 7.90(0.16) |
| Sunspot.5h | 11.71(0.10) | 11.61(0.10) | 11.63(0.10) | 11.66(0.10) | 11.57(0.10) | 11.58(0.10) | 13.74(0.11) | 13.16(0.13) |
| TGauss.3l | 0.02(0.00) | 0.00(0.00) | 0.01(0.00) | 0.02(0.00) | 0.00(0.00) | 0.01(0.00) | 0.02(0.00) | 0.25(0.05) |
| TGauss.3h | 0.24(0.00) | 0.23(0.00) | 0.24(0.00) | 0.21(0.00) | 0.21(0.00) | 0.22(0.00) | 0.23(0.00) | 0.52(0.02) |
| TGauss.5l | 0.16(0.01) | 0.14(0.01) | 0.14(0.00) | 0.18(0.01) | 0.20(0.01) | 0.17(0.01) | 0.31(0.01) | 0.59(0.03) |
| TGauss.5h | 0.66(0.01) | 0.60(0.01) | 0.63(0.01) | 0.56(0.01) | 0.56(0.01) | 0.56(0.01) | 0.83(0.01) | 1.26(0.04) |
| GaussT.2l | 0.56(0.01) | 0.56(0.01) | 0.56(0.01) | 27.69(0.32) | 20.33(0.45) | 16.42(0.47) | 0.82(0.02) | 0.56(0.01) |
| GaussT.2h | 13.06(0.05) | 28.22(0.10) | 33.46(0.12) | 27.50(0.15) | 31.49(0.14) | 30.96(0.15) | 11.58(0.15) | 11.91(0.02) |
| GaussT.3l | 0.11(0.00) | 0.11(0.00) | 0.11(0.00) | 0.16(0.00) | 0.12(0.00) | 0.12(0.00) | 0.17(0.01) | 0.11(0.00) |
| GaussT.3h | 0.68(0.09) | 0.43(0.00) | 0.43(0.00) | 0.40(0.00) | 0.41(0.00) | 0.42(0.01) | 0.48(0.01) | 16.60(0.40) |
| Noiseless.3l | 0.12(0.00) | 0.12(0.00) | 0.11(0.00) | 0.17(0.00) | 0.13(0.00) | 0.12(0.00) | 0.18(0.01) | 0.11(0.00) |
| Noiseless.3h | 0.24(0.00) | 0.24(0.00) | 0.24(0.00) | 0.29(0.00) | 0.26(0.00) | 0.26(0.00) | 0.29(0.00) | 0.24(0.00) |
| Noiseless.5l | 4.51(0.08) | 4.47(0.08) | 4.43(0.08) | 13.80(0.12) | 13.13(0.13) | 13.02(0.13) | 8.23(0.14) | 4.57(0.09) |
| Noiseless.5h | 12.38(0.10) | 12.61(0.10) | 12.60(0.10) | 16.47(0.11) | 16.05(0.12) | 16.04(0.12) | 11.92(0.08) | 12.36(0.10) |

## 6 Plots for the analysis of Dortmund data

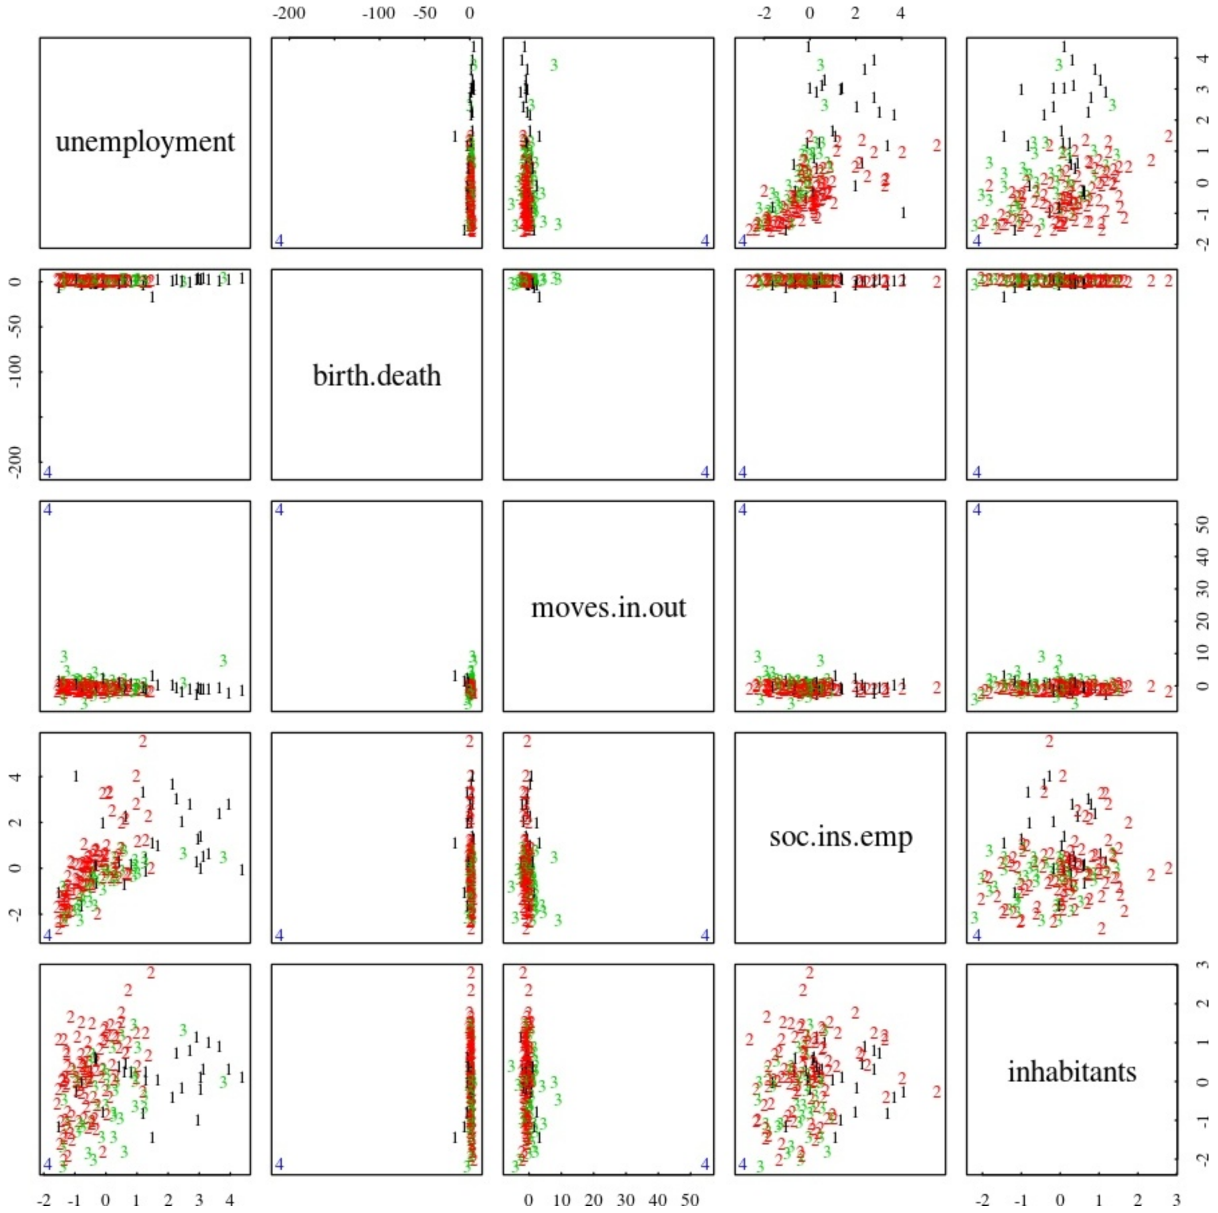


Figure 25: MCLUST clustering without the uniform noise component for the Dortmund data. This clustering is based on a pure Gaussian mixture model.

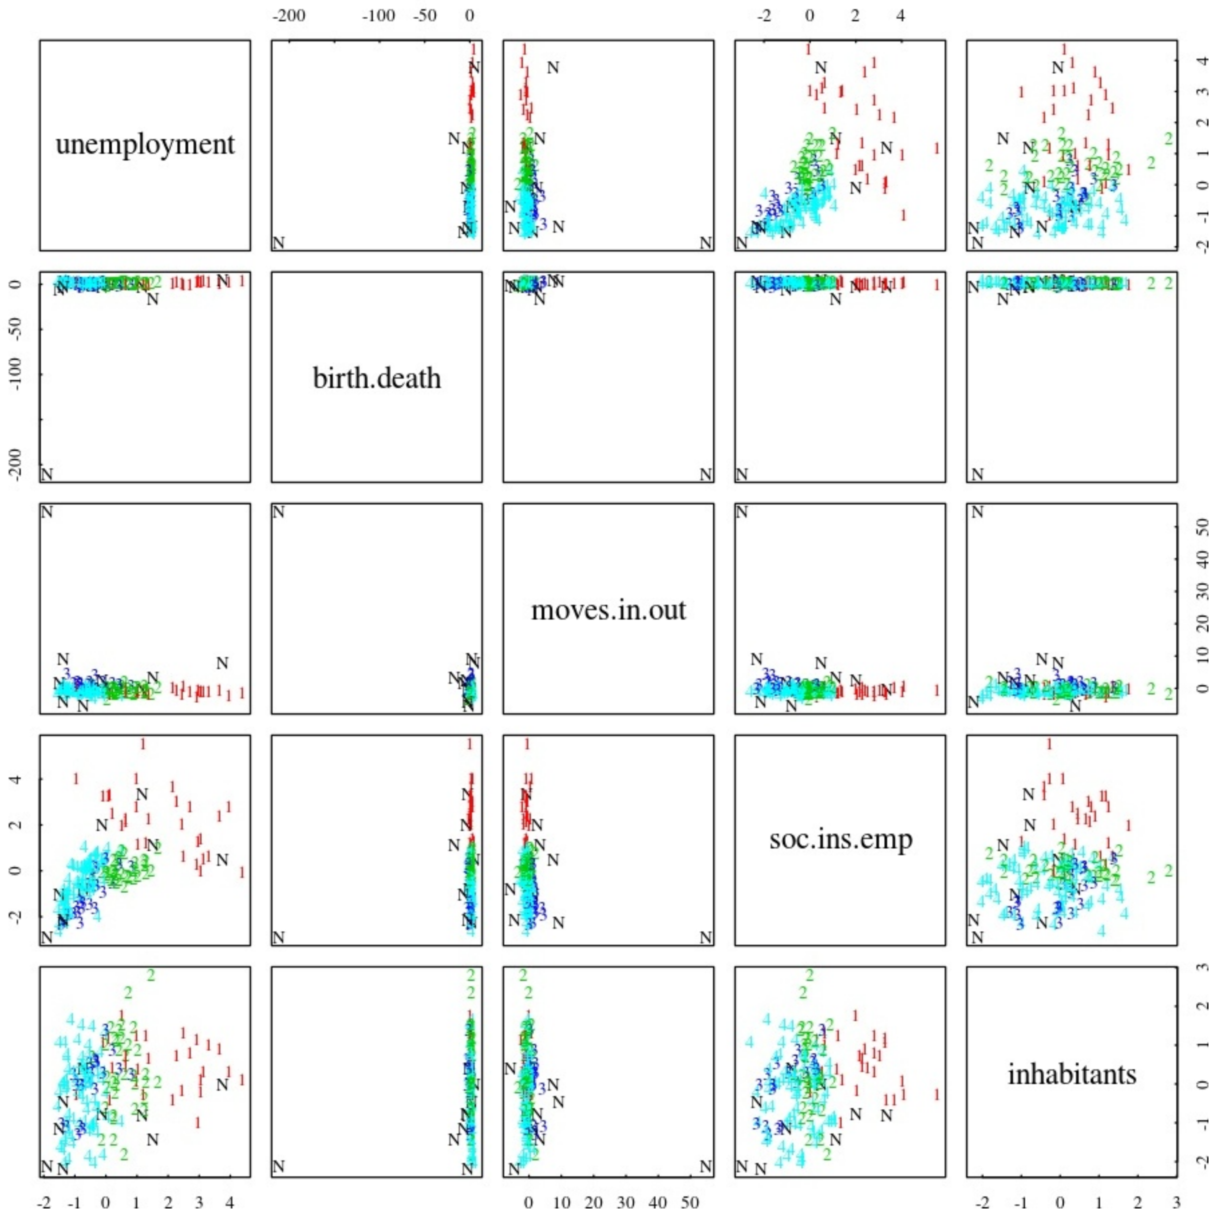


Figure 26: OTRIMLE clustering for the Dortmund data obtained without the penalty term (that is $\beta = 0$).

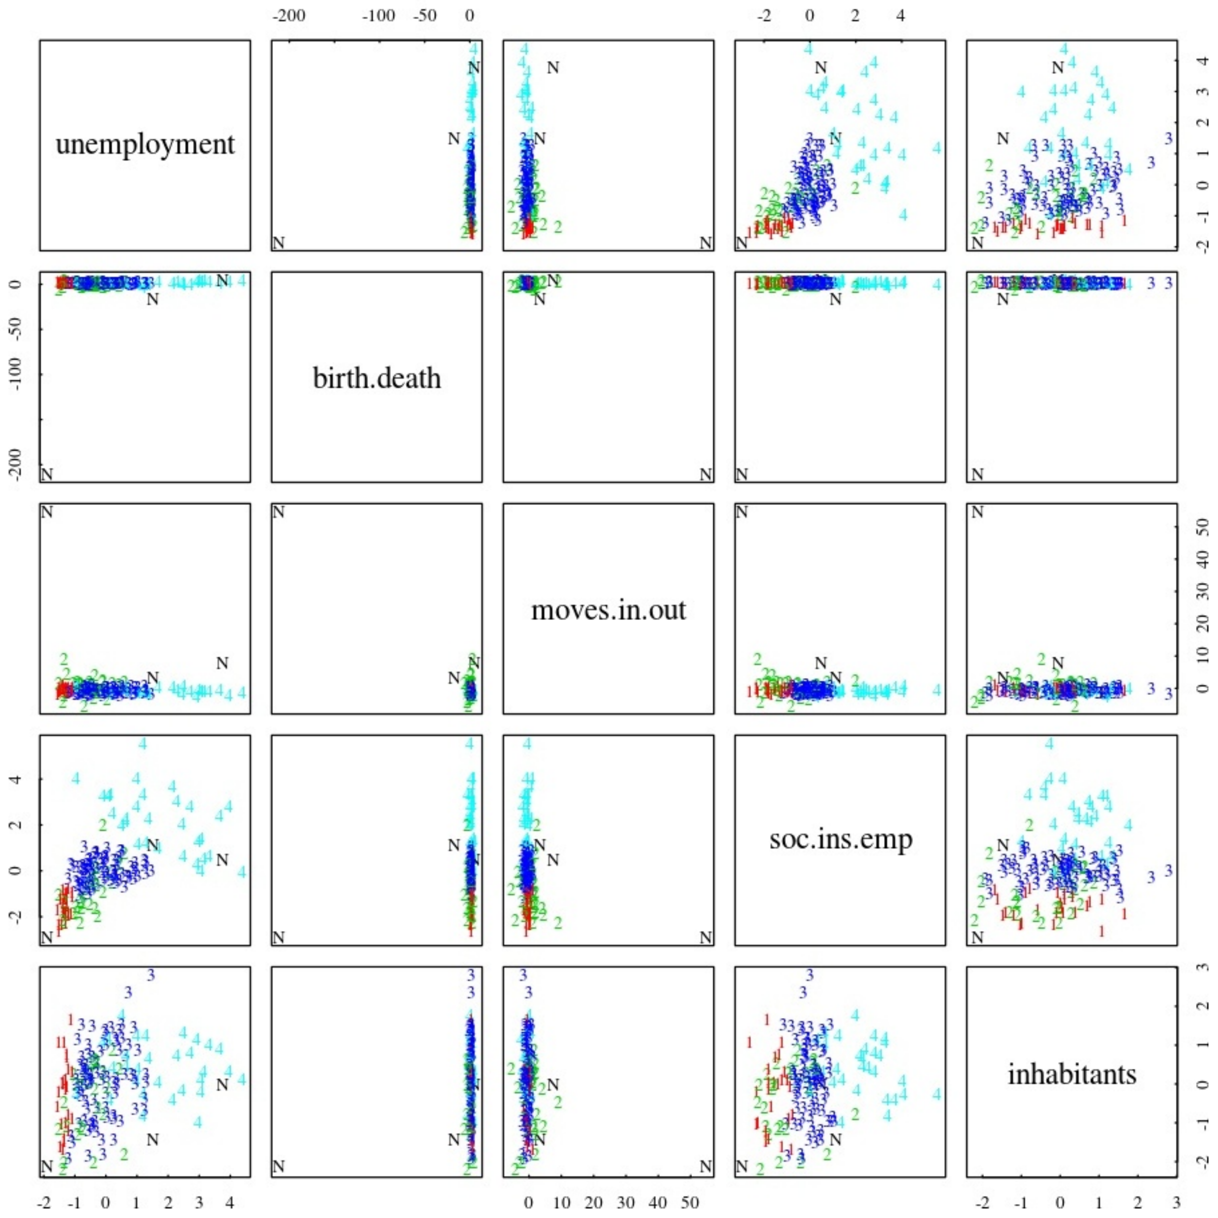


Figure 27: MCLUST clustering with the uniform noise component for the Dortmund data.

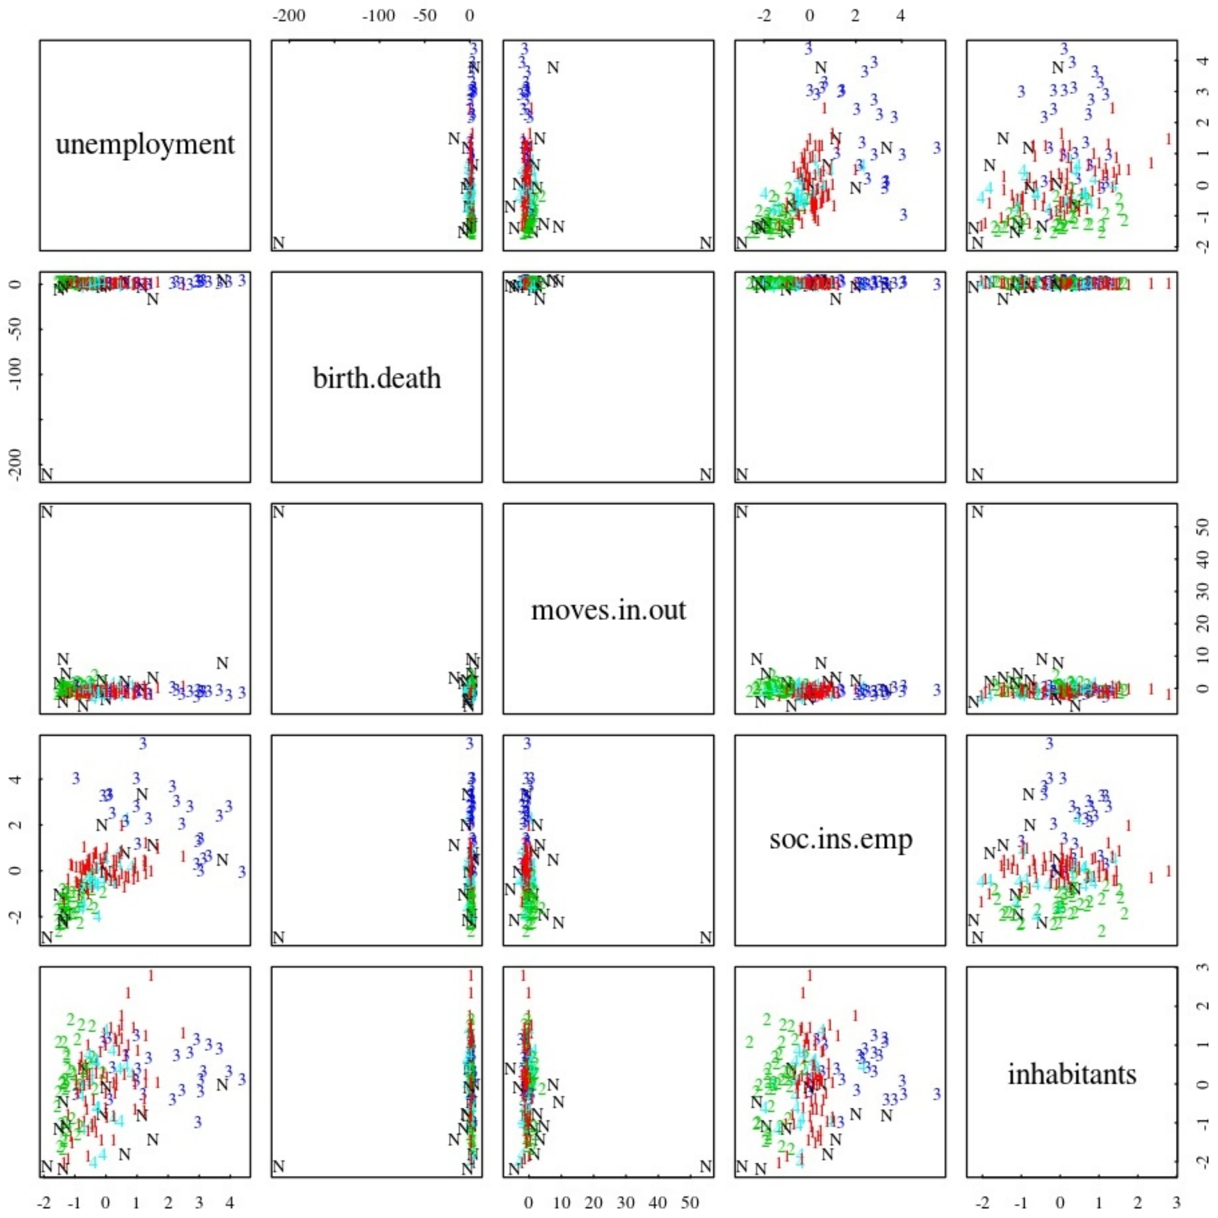


Figure 28: TCLUST clustering for the Dortmund data with trimming level set at 20%.

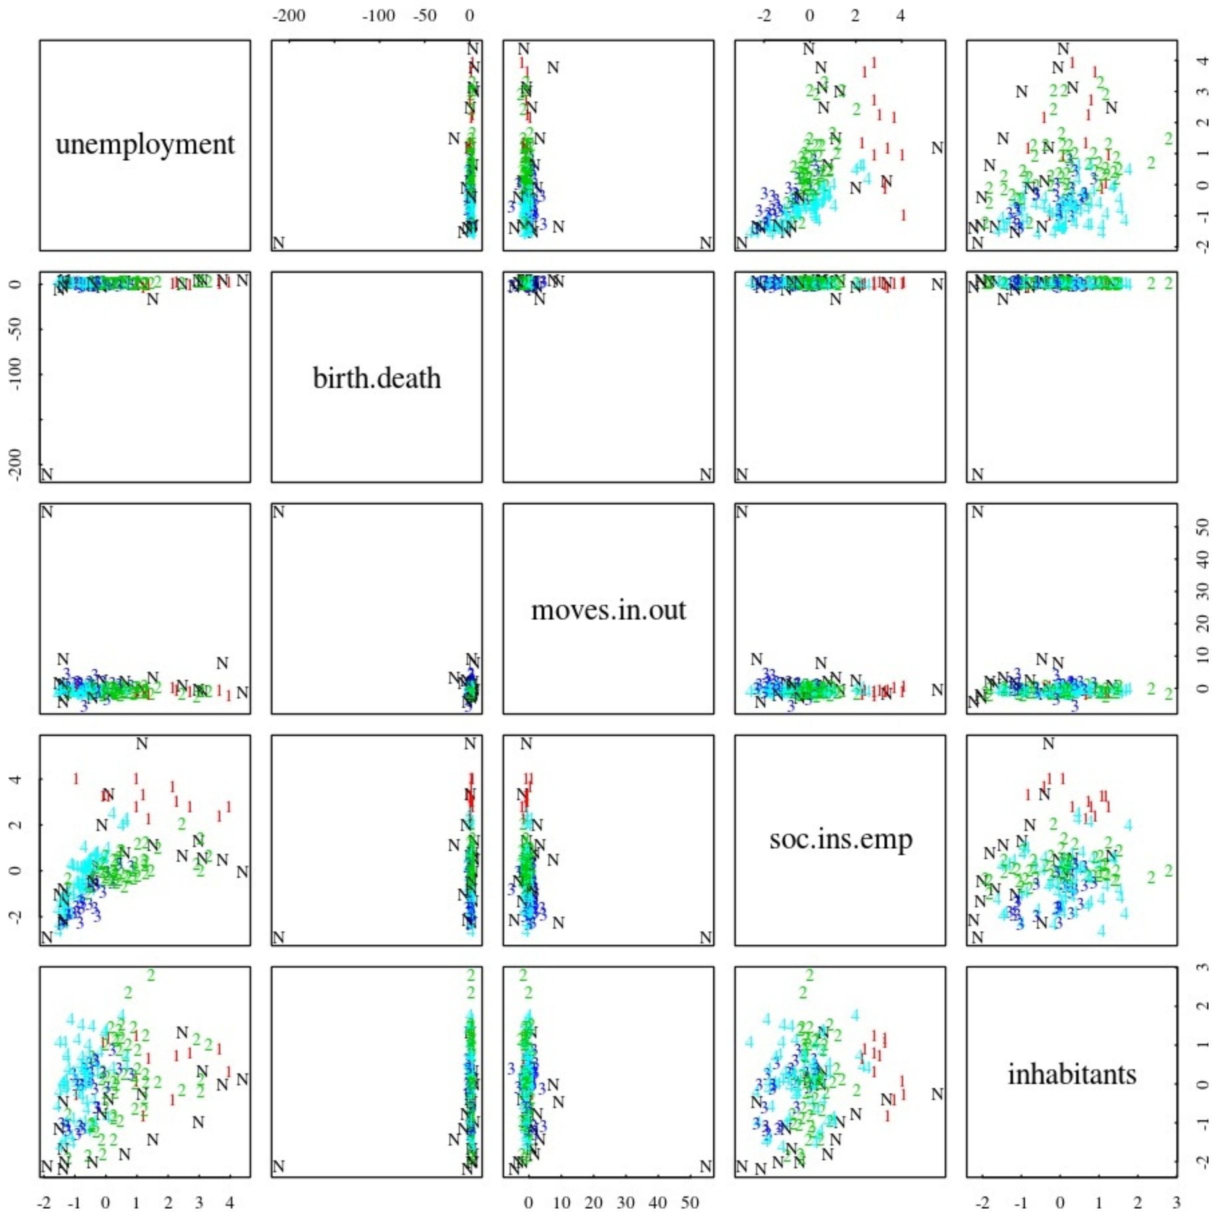


Figure 29: Clustering based on a mixture of Student-t distribution with 4 degrees of freedom for the Dortmund data. Noise identified as in McLachlan–Peel's original proposal. Note that a mixture of $t_4$-distributions was fitted because numerical problems were encountered fitting a $t-$mixture with lower degrees of freedom.

# 7 Information on folk song data

## 7.1 Features

The 18 features were computed by the software "FANTASTIC" (Müllensiefen (2009)). Originally, this software computed 40 features. We discarded some features that were either discrete or partly discrete in a way not compatible with clustering based on continuous distributions. Some more features were discarded because, looking at correlations and scatterplots, they carried almost identical information to some other features. The final list of used features (see Müllensiefen (2009)) was mean.entropy, mean.Yules.K, mean.Sichels.S, p.range, p.entropy, i.abs.mean, i.abs.std, i.entropy, note.dens, tonalness, tonal.clarity, tonal.spike, int.cont.grad.mean, step.cont.glob.dir, step.cont.loc.var, poly.coeff1, poly.coeff2, poly.coeff3. Features were standardized to unit MAD.

## 7.2 Plot

The following plot is a two-dimensional projection of the 18-dimensional folk song data, which was obtained by local discriminant 50-nearest-neighbour based dimension reduction (Hastie and Tibshirani, 1996), discriminating the Luxemburg and Warmia classes, as implemented in the R-package `fpc`.

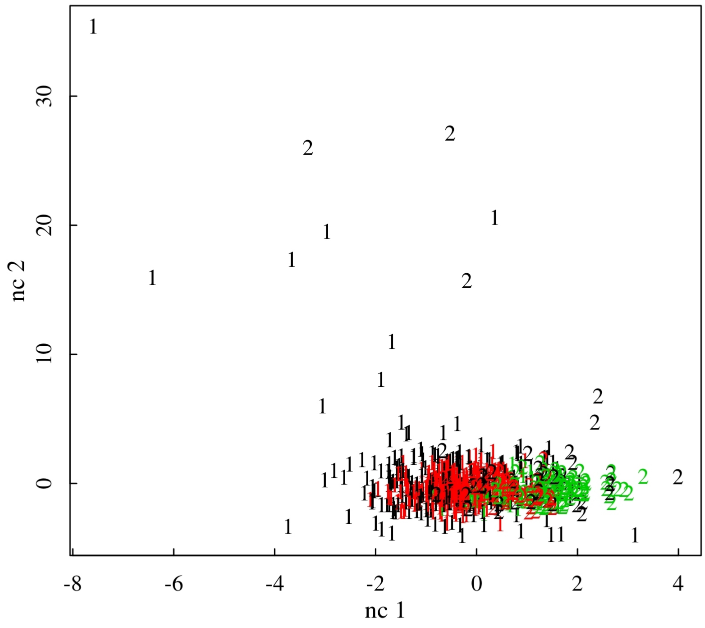


Figure 30: Local neighborhood-based discrimination plot for folk song data with songs from Luxemburg and Warmia denoted by symbols "1" and "2". The OTRIMLE clustering with $\beta = 0$ is indicated by colors red and green for the two clusters and black for points classified as noise.

# References

Banfield, J. D. and A. E. Raftery (1993). Model-based gaussian and non-gaussian clustering. *Biometrics 49*, 803–821.

Biernacki, C., G. Celeux, and G. Govaert (2003). Choosing starting values for the EM algorithm for getting the highest likelihood in multivariate gaussian mixture models. *Computational Statistics & Data Analysis 41*(3), 561–575.

Byers, S. and A. E. Raftery (1998). Nearest-neighbor clutter removal for estimating features in spatial point processes. *Journal of the American Statistical Association 93*(442), 577–584.

Cator, E. A. and H. P. Lopuhaä (2012). Central limit theorem and influence function for the MCD estimators at general multivariate distributions. *Bernoulli 18*(2), 520–551.

Coretto, P. and C. Hennig (2011). Maximum likelihood estimation of heterogeneous mixtures of gaussian and uniform distributions. *Journal of Statistical Planning and Inference 141*(1), 462–473.

Coretto, P. and C. Hennig (2015). Robust improper maximum likelihood: tuning, computation, and a comparison with other methods for robust Gaussian clustering. Preprint included in the submission, also available at http://arxiv.org/pdf/1406.0808.

Cuesta-Albertos, J. A., A. Gordaliza, and C. Matrán (1997). Trimmed k-means: An attempt to robustify quantizers. *Annals of Statistics 25*, 553–576.

Fraley, C., A. E. Raftery, T. B. Murphy, and L. Scrucca (2012). *mclust Version 4 for R: Normal Mixture Modeling for Model-Based Clustering, Classification, and Density Estimation.*

Fritz, H., L. A. García-Escudero, and A. Mayo-Iscar (2012). tclust: An R package for a trimming approach to cluster analysis. *Journal of Statistical Software 47*(12), 1–26.

Gallegos, M. T. (2002). Maximum likelihood clustering with outliers. In *Classification, Clustering, and Data Analysis*, pp. 247–255. Springer.

Gallegos, M. T. and G. Ritter (2005). A robust method for cluster analysis. *Annals of Statistics 33*(5), 347–380.

Gallegos, M. T. and G. Ritter (2013). Strong consistency of $k$-parameters clustering. *Journal of Multivariate Analysis 117*, 14–31.

García-Escudero, L. A., A. Gordaliza, C. Matrán, and A. Mayo-Iscar (2008). A general trimming approach to robust cluster analysis. *Annals of Statistics 38*(3), 1324–1345.

Hastie, T. and R. Tibshirani (1996). Discriminant adaptive nearest neighbor classification. *IEEE Transactions on Pattern Analysis and Machine Intelligence 18*, 607–616.

Hennig, C. (2004). Breakdown points for maximum likelihood estimators of location-scale mixtures. *The Annals of Statistics 32*(4), 1313–1340.

Hennig, C. and B. Hausdorf (2015). *prabclus: Functions for clustering of presence-absence, abundance and multilocus genetic data.* CRAN. R package version 2.2-6.

Karlis, D. and E. Xekalaki (2003). Choosing initial values for the EM algorithm for finite mixtures. *Computational Statistics & Data Analysis 41*(3-4), 577–590.

Kiefer, J. (1953). Sequential minimax search for a maximum. *Proceedings of the American Mathematical Society 4*(3), 502–506.

McLachlan, G. J. and D. Peel (2000a). *Finite Mixture Models.* New York: Wiley.

McLachlan, G. J. and D. Peel (2000b). Robust mixture modelling using the t–distribution. *Statistics and Computing 10*(4), 339–348.

Müllensiefen, D. (2009). *Fantastic: Feature ANalysis Technology Accessing STatistics (In a Corpus): Technical Report v1.5*. London, United Kingdom: Goldsmiths University of London.

Venables, W. N. and B. D. Ripley (2002). *Modern Applied Statistics with S* (Fourth ed.). New York: Springer. ISBN 0-387-95457-0.
